# Supplementary material for: Heterogeneous Quantile Treatment Effect Estimation for Longitudinal Data with High-Dimensional Confounding-v2
Source: arXiv:2508.16326 source file (2026-08-31)
Supplement: Supplementary file 1 [file supplement.tex]

\documentclass[12pt,doublespace]{article}
\usepackage[small,compact]{titlesec}
\usepackage[sectionbib]{natbib}
\usepackage{array,epsfig,rotating}
\usepackage[]{hyperref}  %<----modified by Ivan
%%%%%%%%%%%%%%%%%%%%%%%%%%%%%%%%%%%%
\usepackage{sectsty, secdot}
\renewcommand{\theequation}{\thesection\arabic{equation}}
%\sectionfont{\fontsize{12}{15}\selectfont}

%%%%%%%%%%%%%%%%%%%%%%%%%%%%%%%%%%%%%%%%%%%%%%%%%%%%%%%%%%%%%%%%%%%%%%%%%%%%%%%%%%%%%%%%

\setcounter{totalnumber}{50} \setcounter{topnumber}{50}
\setcounter{bottomnumber}{50}
\renewcommand\arraystretch{1}
\abovecaptionskip 5pt \belowcaptionskip 0pt
\floatsep 5pt    %separation between floats on a page with text
\intextsep 5pt   %separation between floats and the text

%%%%%%%%%%%%%%%%%%%%%%%%%%%%%%
\oddsidemargin 0in \evensidemargin 0in \textwidth      6.1in
\headheight     0in \topmargin      0in \textheight 8in
%%%%%%%%%%%%%%%%%%%%%%%%%%%%%%

\usepackage{amsmath}
\usepackage{amssymb}
\usepackage{amsfonts}
\usepackage{multirow}
\usepackage{amsthm}

\setcounter{page}{1}

\newtheorem{theorem}{Theorem}
\newtheorem{lemma}{Lemma}

\newtheorem{proposition}{Proposition}

\newtheorem{assumption}{Assumption}
\newtheorem{remark}{Remark}

\usepackage[utf8]{inputenc}
\usepackage{indentfirst}
\usepackage{amsthm,amsmath, amssymb}
\usepackage{xcolor} %字体颜色
\usepackage{graphicx} %图片
\usepackage{natbib}
\usepackage{bm}
\usepackage{diagbox}
\usepackage{subfigure}
\usepackage{booktabs}
\usepackage{multirow}
\numberwithin{equation}{section}
\def\BT{\mathbf{T}}
\def\BW{\mathbf{W}}
\def\BX{\mathbf{X}}
\def\Bd{\mathbf{d}}
\def\Bx{\mathbf{x}}
\def\BZ{\mathbf{Z}}
\def\BL{\mathbf{L}}
\def\Bbeta{\boldsymbol{\beta}}
\def\Btheta{\boldsymbol{\theta}}
\def\Bzeta{\boldsymbol{\zeta}}
\def\Bdelta{\boldsymbol{\delta}}
\def\Bpsi{\boldsymbol{\psi}}
\def\Bxi{\boldsymbol{\xi}}
\def\Bell{\boldsymbol{\ell}}
\def\BSigma{\boldsymbol{\Sigma}}
\def\Bmeta{\boldsymbol{\eta}}
\def\BD{\mathbf{D}}
\def\BJ{\mathbf{J}}
\def\Be{\mathbf{e}}
\def\Ba{\mathbf{a}}
\def\Bb{\mathbf{b}}

%%%%%%%%%%%%%%%%%%%%%%%%%%%%%%%%%%%%%%%%%%%%%%%%%%%%%%%%%%%%%%%%%%%%%%%%%%%%%%%%%%%%%%%%%%%%%%%%%%%%%%%%%%%%%%%%%%%%%%%%%%%%
\definecolor{zhixin}{rgb}{0.6, 0.2, 0.8}
\definecolor{yanlin}{rgb}{0.8, 0.0, 0.0}

%%%%%%%%%%%%%%%%%%%%%%%%%%%%%%%%%%%%%%%%%%%%%%%%%%%%%%%%%%%%%%%%%%%%%%%%%%%%%%%%%%%%%%%%%%%%%%%%%%%%%%%%%%%%%%%%%%%%%%%%%%%%
%%%%%%%%%%%%%%%%%%%%%%%%%%%%%%%%%%%%%%%%%%%%%%%%%%%%%%%%%%%%%%%%%%%%%%%%%%%%%%%%%%%%%%%%%%%%%%%%%%%%%%%%%%%%%%%%%%%%%%%%%%%%

\begin{document}

\title{{\bf Web-Based Supplementary Materials for ``Heterogeneous Quantile Treatment Effect Estimation for Longitudinal Data with High-Dimensional Confounding"}}
\author{by Zhixin Qiu, Huichen Zhu, Wenjie Wang and Yanlin Tang}
\date{}
\maketitle

\appendix
\renewcommand{\thetable}{S.\arabic{table}}
\renewcommand{\thetheorem}{S.\arabic{theorem}}
\renewcommand{\thesection}{S\arabic{section}}
\renewcommand{\theproposition}{S.\arabic{proposition}} 
\setcounter{table}{0}
\renewcommand{\theequation}{S.\arabic{equation}} 
\setcounter{equation}{0}
\renewcommand{\thelemma}{S.\arabic{lemma}} 
\setcounter{lemma}{0}

The Web-Based Supplementary Materials include four parts, Section S1 for regularity assumptions and theoretical results for estimated nuisance parameters, Section S2 for additional simulation studies, Section S3 for proof of orthogonality, and Section S4 for the detailed proof of the theoretical results.

\section{Regularity Assumptions and Theoretical Results for Nuisance Parameters}\label{Assumptions and Additional Theoretical Results}
\subsection{Regularity Assumptions}
We ensure good statistical behavior by adopting the honesty principle \citep{wager2018estimation}, which has been proven to be effective in the forest-based regression literature.
Concretely, each tree is grown on a subsample $\mathcal S$ of size $s$ drawn without replacement from the full cohort of $n$ subjects, with $s/n \to 0$ and $s \to \infty$.
The subsample is then randomly partitioned into two disjoint subsets $\mathcal S_1$ and $\mathcal S_2$: $\mathcal S_1$ is used solely to determine the split locations, whereas $\mathcal S_2$ is used for estimation. 
This strict separation between model selection and estimation eliminates bias in the estimated treatment effects and underpins the theoretical guarantees of our procedure.

The following Assumptions~\ref{tree assumption}-\ref{assum:design_subgaussian} are needed for the theoretical derivation of the nuisance parameters, and Assumptions~\ref{A3.5}-\ref{sparsity level} are additional ones for the theoretical properties of the treatment effect estimator.

\begin{assumption}\label{tree assumption}
In each split, at least a fraction $0<\rho \leq 0.2$ of the subjects in $\mathcal S_2$ falls into each child node. There are between $r$ and $2r-1$ subjects from $\mathcal S_2$ at each leaf of the tree, with $r=O(1)$. Furthermore, in each split, every feature has a splitting probability of at least $\pi/p_x$, for some constant $0 < \pi < 1$.
\end{assumption}

\begin{assumption}\label{assum:design_matrix}
    Let $\bm\Sigma = \mathbb E[\BD_{ij}\BD_{ij}^\top]$.  Its eigenvalues satisfy
    \[
      0 \;<\;\sigma_{\min}\;\le\;\lambda_{\min}(\bm\Sigma)
      \;\le\;\lambda_{\max}(\bm\Sigma)\;\le\;\sigma_{\max}\;<\;\infty.
    \]
     % The eigenvalues of the conditional covariance matrix $\bm{\Sigma}=\mathbb{E}\left[\BD_{ij}\BD_{ij}^{\top}\right]$ satisfies $0<\sigma_{min}<\sigma_1\leq\sigma_2\leq\cdots\leq\sigma_{p+q}\leq\sigma_{max}<\infty.$
\end{assumption}

\begin{assumption}\label{assum:coeff}
Both the true $\Bell^{*(\nu)}(\Bx)$ $(\nu=1,\dots,p_t)$ and $\Bzeta^*_\tau(\Bx)$ are $k$‐sparse and $L$‐Lipschitz in $\Bx$.  That is,
    \[
      \|\Bell^{*(\nu)}(\Bx)\|_0\le k,
      \quad
      \|\Bell^{*(\nu)}(\Bx_1)-\Bell^{*(\nu)}(\Bx_2)\|_2\le L\|\Bx_1-\Bx_2\|,
    \]
    and similarly for $\Bzeta^*_\tau(\cdot)$.
    % The coefficient $\Bell^{\star(\nu)}(\Bx)$, $(\nu=1,2,\dots,q)$ and $\Bzeta^{\star}_\tau(\Bx)$ are $k$-sparse and $L$-Lipschitz continuous with respect to $\Bx$.
\end{assumption}

\begin{assumption}\label{assum:density}
    Let $f(y\mid\Bd,\Bx)$ be the conditional density of $Y\mid\BD = \Bd, \BX = \Bx$.
    \begin{enumerate}
        \item \textbf{Smoothness.} $f(y\mid\Bd,\Bx)$ is bounded and continuously differentiable in $y$ with 
        \[
        \sup_{y,\Bd,\Bx}\bigl|f(y\mid\Bd,\Bx)\bigr|\le \bar f,
        \quad
        \sup_{y,\Bd,\Bx}\Bigl|\frac{\partial}{\partial y}f(y\mid\Bd,\Bx)\Bigr|\le \bar f'.
      \]
      \item \textbf{Nondegeneracy.} Let $\Gamma$ be a compact subset of (0,1). For every $\tau\in\Gamma$ and design vector $\Bd$,
  \[
    f\bigl(\Bzeta^*_\tau(\Bx_0)^\top \Bd \mid \Bd,\Bx_0\bigr)
      \;\ge\;\underline f \;>\;0.
  \]
    \end{enumerate}
    % is continuously differentiable in $Y$, $f(Y\mid\BD,\BX)$ and $\frac{\partial}{\partial Y}f(Y\mid\BD,\BX)$  are bounded in absolute value by constants $\bar{f}$ and $\bar{f}'$ respectively, uniformly in $Y\in\mathbb{R}$ and $\BD$, $\BX$ in the support.  Moreover, the conditional density of $Y_i$ evaluated at the conditional quantile $\Bzeta^{\star}_\tau(\Bx_0)^{\top}\BD_{ij}$ is bounded away from zero uniformly in $\tau\in\Gamma$ and $\BD_{ij}$ in the support , that is $f(\Bzeta^{\star}_\tau(\Bx_0)^{\top}\BD_{ij}\mid\BD_{ij},\Bx_0)>\underline{f}>0$.
\end{assumption}

\begin{assumption}\label{assum:kernel_function}
    The kernel function $K:\mathbb{R}\rightarrow[0,\infty)$ is symmetric around zero and satisfies $\int_{-\infty}^\infty K(u)du=1$, $\int_{-\infty}^\infty u^2K(u)du<\infty$, $\kappa_l=\min_{|u|\leq 1}K(u)>0$.
\end{assumption}

\begin{assumption}\label{assum:design_subgaussian}
    Define $\widetilde\BD_{ij} = \bm\Sigma^{-1/2}\,\BD_{ij}$. We assume the following conditions for $\BD_{ij}$.
    \begin{enumerate}
        \item \textbf{Sub-Gaussian.} There exist constants $v_0,c_0\ge1$ such that, for all $\mathbf{u}\in\mathbb R^{p_t+p_w}$ and $t\ge0$,
         \[
         \Pr\bigl(|\widetilde\BD_{ij}^\top \mathbf{u}|\ge v_0\|\mathbf{u}\|_2\,t\bigr)\;\le\; c_0\,e^{-t^2}.
        \]
      \item For all vectors $\mathbf{a},\mathbf{b}\in\mathbb{R}^{p_t+p_w}$, the random variables $\left|\BD_{ij}^{\top}\mathbf{a}\right|$ and $\left|\BD_{ij}^{\top}\mathbf{b}\right|$ are non-negatively correlated.
    \end{enumerate}
    % $\widetilde{\BD}_{ij}=\bm{\Sigma}^{-1/2}\BD_{ij}$ is sub-Gaussian: there exists constants $v_0, c_0\geq1$ such that $\mathbb{P}\left(|\widetilde{\BD}_{ij}^{\top}\bm{u}|\geq v_0^2\left\|\bm{u}\right\|_2\cdot t\right)\leq c_0e^{-t^2}$ for all $\bm{u}\in\mathbb{R}^{p+q}$ and $t\geq0$.
\end{assumption}

\begin{assumption}\label{A3.5}
The heterogeneous treatment effect vector $\Btheta^{\star}(\Bx)$ is $L$-Lipschitz continuous in $\Bx$.
\end{assumption}

\begin{assumption}\label{A3.6}
The cumulative distribution function $F\left(\BT\mid\BW,\BX\right)$ is $L$-Lipschitz continuous in $\BT$. Moreover, recall that $\Be$ denotes the error term of $\BT$, with each component having a finite second moment.
\end{assumption}
	
\begin{assumption}\label{A3.7}
		For any weights $\{\alpha_i(\Bx_0)\}$ with $\sum_{i\in\mathcal{D}_2}\alpha_i(\Bx_0)=1$ and $\alpha_i(\Bx_0)\geq0$, the estimating equation $\arg\min_{\Btheta}\|\sum_{i\in\mathcal{D}_2}\alpha_i(\Bx_0)\sum_{j=1}^{m_i}\frac{1}{m_i}\psi(\BZ_{ij};\Btheta,\widehat{\Bmeta}(\Bx_0))\|$ returns a minimizer $\widehat{\Btheta}(\Bx_0)$ that satisfies $\|\sum_{i=1}^n\alpha_i(\Bx_0)\sum_{j=1}^{m_i}\frac{1}{m_i}\psi(\BZ_i;\widehat{\Btheta}(\Bx_0),\widehat{\Bmeta}(\Bx_0))\|\leq C\max_i\{\alpha_i(\Bx_0)\}$ for some constant $C\geq0$.
\end{assumption}
    
\begin{assumption}\label{sparsity level}
    Suppose the sparsity level $k$ satisfies $k\leq \min\left\{s^{1/(4\omega p_x)},\frac{\left(n/s\right)^{1/4}}{\sqrt{\log(p_t+p_w)}}\right\}$, where $\omega=\frac{\log(\rho^{-1})}{\pi\log((1-\rho)^{-1})}$, with $\rho$ and $\pi$ defined in Assumption \ref{tree assumption}.
\end{assumption}

Assumption~\ref{tree assumption} is a commonly used assumption in the random forest literature \citep{wager2018estimation, athey2019generalized,pmlr-v97-oprescu19a}, which ensures the kernel shrinkage property.
Assumptions~\ref{assum:design_matrix}-\ref{assum:design_subgaussian} underpin theoretical analysis of the two nuisance estimators $\widetilde{\BL}(\Bx_0)$ and $\widetilde{\Bbeta}_{\tau h}(\Bx_0)$ defined in (7) and (8) in Section 2.4 of the main article. 
Assumption~\ref{assum:design_matrix} ensures that the population design matrix has eigenvalues bounded away from zero and infinity. This assumption guarantees the identifiability and numerical stability of the Lasso-type estimators. 
Assumption~\ref{assum:coeff} is a mild sparsity and smoothness condition. 
Assumption~\ref{assum:density} imposes regularity conditions on the conditional density of the response variable $Y_{ij}$ given $\BD_{ij}$, which is common in the literature. 
Assumption \ref{assum:kernel_function} is a standard regularity condition on the kernel function, these conditions are mild and satisfied by most commonly used kernels (e.g., Gaussian, Epanechnikov, uniform).
The first part of Assumption \ref{assum:design_subgaussian} is a commonly used assumption. The second part is somewhat strong, but can be verified when $\BD_{ij}$ follows a multivariate normal distribution. We will discuss this condition in detail in Remark~\ref{validity of assum} later. 
To derive the theoretical results for treatment effect estimation, Assumptions~\ref{A3.5}-\ref{sparsity level} are needed. Assumptions~\ref{A3.5}-\ref{A3.7} are used to provide the consistency of the target estimator $\widehat{\Btheta}(\Bx_0)$. Assumptions~\ref{A3.5} and \ref{A3.6} are regular conditions that require both heterogeneous treatment effects and a conditional cumulative distribution of the outcome given confounders and modifiers to be Lipschitz continuous. Assumption~\ref{A3.7} imposes the existence of an approximate solution of equation (4), which is a common assumption in random forests \citep{athey2019generalized}. To establish the convergence rate of treatment effect estimator, we impose Assumption~\ref{sparsity level} to restrict the sparsity level of the nuisance parameters.

\begin{remark}{\textbf{(Validity of the Second Condition in Assumption~\ref{assum:design_subgaussian})}}\label{validity of assum}
We can prove that $\BD_{ij}$ following the multivariate normal distribution is a sufficient condition for the second part of Assumption~\ref{assum:design_subgaussian}. 
Suppose that $\BD_{ij}\sim N(\mathbf{0},\BSigma_{\BD})$, and denote the correlation between $\BD_{ij}^{\top}\Ba$ and $\BD_{ij}^{\top}\Bb$ as $\rho:=\frac{\Ba^{\top}\BSigma_{\BD}\Bb}{\sqrt{\Ba^{\top}\BSigma_{\BD}\Ba}\sqrt{\Bb^{\top}\BSigma_{\BD}\Bb}}$. \cite{kamat1953incomplete} indicates that
$$\mathrm{Corr}\left(\left|\BD_{ij}^{\top}\Ba\right|,\left|\BD_{ij}^{\top}\Bb\right|\right)=\frac{2}{\pi}\left\lbrace\sqrt{1-\rho^2}+\rho\arcsin(\rho)-1\right\rbrace\geq 0.$$
\end{remark}

\subsection{Theoretical Results for Nuisance Parameters}\label{Nuisance-property}
In the following, we present the theoretical properties of the nuisance parameters. We begin by introducing the kernel shrinkage proposition, which guarantees that the similarity weights are positive only for points lying within a small neighborhood of $\Bx_0$. This localization property will play a key role in our subsequent analysis.
\begin{proposition}{\textbf{(Kernel shrinkage, Theorem 3.2 in \citealp{wager2018estimation})}}\label{thm:shrinkage}
Suppose that the tree satisfies Assumption~\ref{tree assumption}. Furthermore, the distribution of $\BX$ admits a density in $[0, 1]^{p_x}$ that is bounded away from both zero and infinity. Then the tree weights satisfy 
\begin{eqnarray}
\mathbb{E}\left[\sup\{\|\Bx_0-\BX_i\|: \alpha_{ib}(\Bx_0)> 0\}\right] = O(s^{-\frac{1}{2\omega p_x}}),\notag
\end{eqnarray} 
where $\omega$ is defined in Assumption \ref{sparsity level}.
\end{proposition}

Then we establish nonasymptotic error bounds for our nuisance estimators. Proposition~\ref{thm:nuisance_error} provides theoretical guarantee for $\widetilde{\BL}(\Bx_0)$ and Theorem~\ref{thm_conv} does so for $\widetilde{\Btheta}_{\tau h}(\Bx_0)$.
\begin{proposition}\label{thm:nuisance_error}
\noindent Under Assumptions~\ref{tree assumption}-\ref{assum:coeff}, and assume that $\frac{\lambda_1^{(\nu)}}{n_{rf}}\geq 2\left(Ls^{-\frac{1}{2\omega d}}+\sqrt{\frac{s\log (p_w/\gamma)}{n}}\right)$ for some $0<\gamma<1$, then with probability $1-\gamma$, $\|\widetilde{\Bell}^{(\nu)}(\Bx_0)-\Bell^{\star(\nu)}(\Bx_0)\|\leq\frac{2\lambda_1^{(\nu)} k}{n_{rf}\left(\sigma_{\text{min}}-32\sqrt{\frac{s\log(p_w/\gamma)}{n}}\right)}$, $k$ is the sparsity level as defined in Assumption~\ref{assum:coeff} and $\omega$ is defined in Assumption~\ref{sparsity level}, $\nu=1,2,\dots,p_t$.
\end{proposition}
The proof follows directly from that of Theorem 5.2 in \cite{pmlr-v97-oprescu19a}. In practice, we let $\frac{\lambda_1}{n_{rf}}=\frac{c}{100}\sqrt{\frac{s\log p_w}{n}}$, where the constant $c$ is selected from $\left\lbrace1,2,\dots,10\right\rbrace$ using BIC.

\begin{theorem}{\textbf{(Convolution Smoothing)}}\label{thm_conv}
    \noindent Under assumptions \ref{tree assumption}-\ref{assum:design_subgaussian}, the bandwidth $h$ satisfies $\frac{\underline{f}}{4\bar{f}'}\geq\frac{h}{4}\geq C_1s^{-\frac{1}{2\omega p_x}}$, where $C_1=\sigma_{\text{max}}v_0L$ is a constant, $\omega$ is as in Assumption~\ref{sparsity level} and $v_0$ is as in Assumption~\ref{assum:design_subgaussian}. We further assume the penalty level satisfies $\frac{\lambda_2}{n_{rf}}> \bar{f}C_1\sqrt{\log\left(c_0/\gamma\right)}s^{-\frac{1}{2\omega p_x}}+C_2h^2+C_3\sqrt{\frac{s\log\left(\left(p_t+p_w \right)/\gamma  \right) }{n}}$ for constants $\gamma$, $C_2$, $C_3>0$ and $n>s^{1+\left\lbrace 1/(2\omega p_x)\right\rbrace}$, then with probability $1-2\gamma$, 
    $$\left\| \widetilde{\Bzeta}_{\tau h}(\Bx_0)-\Bzeta^{\star}_\tau(\Bx_0)\right\|\leq \frac{1+c}{c\widetilde{\kappa}}\cdot\left(\frac{k}{\sigma_{\text{min}}}\right)^{1/2}\cdot\frac{\lambda_2}{n_{rf}},$$
    where $\widetilde{\kappa}=\kappa_l\left(\frac{9\underline{f}\left(1-c_0e^{-1}\right)}{32}-\sqrt\frac{s\log(1/\gamma)}{nh^2}-\frac{Ls^{-\frac{1}{2\omega p_x}}}{h}\right)$ and $k$ is the sparsity level as defined in Assumption~\ref{assum:coeff}. 
\end{theorem}
Under proper choice of penalty level $\lambda_2$ when $\frac{\lambda_2}{n_{rf}}=O\left( s^{-\frac{1}{2\omega p_x}}+\sqrt{\frac{s\log\left(p_t+p_w \right)  }{n}}\right)$ and the bandwidth $h$ satisfies $O\left(Ls^{-\frac{1}{\omega p_x}}+\frac{s\log\left(1/\gamma\right)}{n}\right)\lesssim h^2\lesssim O\left( Ls^{-\frac{1}{2\omega p_x}}+\sqrt{\frac{s\log\left(p_t+p_w \right) }{n}}\right)$, $\widetilde{\Bzeta}_{\tau h}(\Bx_0)$ achieves the convergence rate $\sqrt{k}\cdot s^{-\frac{1}{2\omega p_x}}+\sqrt{\frac{ks\log\left(p_t+p_w\right) }{n}}$. In practice, we select $\lambda_2$ using the data-driven procedure described in Section 2.4, which ensures $\frac{\lambda_2}{n_{rf}}=O\left( s^{-\frac{1}{2\omega p_x}}+\sqrt{\frac{s\log\left(p_t+p_w \right) }{n}}\right)$. We choose $h$ as $\max\left\lbrace\frac{\sqrt{\tau(1-\tau)}}{3}\left(\frac{s\log (p_t+p_w)}{n}\right)^{1/4},0.1\right\rbrace$.

An alternative method to estimate $\Bbeta_\tau^{\star}(\Bx_0)$ is $\ell_1$-QR without smoothing,
    \begin{equation}\label{eq:beta_nc}
     \widetilde{\Bzeta}_{\tau 0}(\Bx_0)\in\mathop{\arg\min}_{\Bzeta}\left\lbrace\sum_{\{i:i\in\mathcal{D}_1\}}\alpha_i(\Bx_0)\sum_{j=1}^{m_i}\frac{1}{m_i}\rho_{\tau}(Y_{ij}-\Bzeta^{\top}\BD_{ij})+\frac{\lambda_{2}}{n_{rf}}\|\Bzeta\|_1\right\rbrace.
 \end{equation}
By Theorem~\ref{thm:beta_nonsmooth}, the convergence rate of $\widetilde{\Bbeta}_{\tau0}(\Bx_0)$ is slower than that of the convolution-smoothed estimator $\widetilde{\Bbeta}_{\tau h}(\Bx_0)$; \textbf{the slower convergence rate is insufficient to yield the error bound and asymptotic normality of $\widehat{\Btheta}(\Bx_0)$} in the main article. Numerical results in Section~\ref{Additional Simulation} demonstrate that, using $\widetilde{\Bbeta}_{\tau0}(\Bx_0)$ from \eqref{eq:beta_nc} still yields good finite sample performance in estimating the treatment effects. 

When we use $\ell_1-$penalized quantile loss function \eqref{eq:beta_nc} to estimate the nuisance parameter $\Bbeta^{\star}_\tau(\Bx_0)$, we further assume the restricted identifiability condition instead of Assumptions \ref{assum:kernel_function} and \ref{assum:design_subgaussian}.

\setcounter{assumption}{5} 
\renewcommand{\theassumption}{\arabic{assumption}$^\ast$}
\begin{assumption}\label{assum:design_subgaussian'}
	Denote $S$ as the support of $\Bzeta^{\star}_\tau(\Bx_0)$. Define the set $A(e_0):= \{\Bdelta\in\mathbb{R}^{(p_t+p_w)}:\|\Bdelta_{S^c}\|_1\leq e_0\|\Bdelta_{S}\|_1\}$, where $e_0>1,$ $S^C(\Bdelta,m)$ as the support of the $m$ largest in absolute value components of the vector $\Bdelta$ outside  the support of $\Bzeta_\tau(\Bx_0)$.
	For some constants $m\geq0$ and $c_0\geq9$, the matrix $\mathbb{E}\left[\BD_{ij}\BD_{ij}^{\top}\mid\Bx_0\right]$ satisfies
	$$t^2_m:=\inf_{\Bdelta\in A(e_0),\Bdelta\neq0}\frac{\Bdelta^{\top}\mathbb{E}\left[\BD_{ij}\BD_{ij}^{\top}\mid\Bx_0\right]\Bdelta}{\|\Bdelta_{S\cup S^C(\Bdelta,m)}\|^2}>0$$
	and $\log(\underline{f}k_0^2)\leq C_f\log(n\vee (p_t+p_w))$ for some constant $C_f$. Moreover,
	$$t=\frac{3}{8}\frac{\underline{f}^{3/2}}{\overline{f}'}\inf_{\Bdelta\in A(e_0),\Bdelta\neq0}\frac{\mathbb{E}\left[\left|\Bdelta^{\top}\BD_{ij}\right|^2\mid\Bx_0\right]^{3/2}}{\mathbb{E}\left[\left| \Bdelta^{\top}\BD_{ij}\right| ^3\mid\Bx_0\right]}>0.$$
\end{assumption}
\renewcommand{\theassumption}{\arabic{assumption}}

 \begin{theorem}\label{thm:beta_nonsmooth}
		\noindent Under Assumptions \ref{tree assumption}-\ref{assum:density} and \ref{assum:design_subgaussian'}, suppose that the penalty level satisfies $\frac{1}{c}\frac{\lambda_2}{n_{rf}}\geq\sqrt{k}\bar{f}Ls^{-\frac{1}{2\omega p_x}}+\sqrt{\frac{s\log\left(\left(p_t+p_w \right)/\gamma  \right) }{n}}$ for constants $c>1$ and $\gamma>0$, where $\omega$ is defined in Assumption~\ref{sparsity level} and the sparsity level $k$ obeys the growth condition
		\begin{equation}\label{eq18}
			2t\geq\frac{\lambda_2}{n_{rf}}\frac{\sqrt{k} }{\underline{f}^{1/2}t_0}+\sqrt{\frac{\lambda_2^2}{n_{rf}^2}\frac{k }{\underline{f}t_0^2}+Ls^{-\frac{1}{2\omega p_x}}+\left(\frac{s\log\left( 1/\gamma\right)}{n}\right)^{1/2}},
		\end{equation}
  with $t_0$ is defined in Assumption \ref{assum:design_subgaussian'} as $t^2_0:=\inf_{\Bdelta\in A(e_0),\Bdelta\neq0}\frac{\Bdelta^\top\mathbb{E}\left[\BD_i\BD_i^{\top}|\Bx_0\right]\Bdelta}{\|\Bdelta_{S}\|^2}.$
		Then with probability $1-2\gamma$, 
        \begin{equation}\label{eq19}
            \left\| \widetilde{\Bzeta}_{\tau0}(\Bx_0)-\Bzeta^{\star}_\tau(\Bx_0)\right\|\leq\frac{1+\frac{c+1}{c-1}\sqrt{k/m}}{t_m} \left( \kappa_1+\kappa_2\right) ,
        \end{equation}
		where $\kappa_1= \frac{\lambda_2}{n_{rf}}\frac{\sqrt{k} }{\underline{f}t_0}$, $\kappa_2=O\left(s^{-\frac{1}{4\omega p_x}}+\left(\frac{s\log\left( 1/\gamma\right)}{n}\right)^{1/4} \right).$
	\end{theorem}

Note that $s^{-\frac{1}{2\omega p_x}}<\sqrt{\frac{s\log\left(\left(p_t+p_w\right)/\gamma  \right) }{n}}$, our choice of $\lambda_2$ described in Section 2.1 satisfies $\frac{\lambda_2}{n_{rf}}\geq\left\|\sum_{i=1}^n\alpha_i(\Bx_0)\sum_{j=1}^{m_i}\frac{1}{m_i}S_{ij}\left(\Bzeta^{\star}_\tau(\BX_i)\right)\BD_i\right\|_\infty$ with probability $0.9$. Under proper choice of $\lambda_2$, the term $\kappa_2$ in \eqref{eq19} dominates the $\ell_2$-error bound of $\widetilde{\Bzeta}_{\tau0}(\Bx_0)$. Then the result in \eqref{eq19} can be simplified to, with probability $1-2\gamma$,
\begin{equation}
    \left\| \widetilde{\Bzeta}_{\tau0}(\Bx_0)-\Bzeta^{\star}_{\tau}(\Bx_0)\right\|=O\left(s^{-\frac{1}{4\omega p_x}}+\left(\frac{s\log(1/\gamma)}{n}\right)^{1/4}\right).
\end{equation}

\section{Additional Simulation Results}\label{Additional Simulation}
\subsection{Performance Comparison of \textbf{OQRF} and \textbf{OQRF-nc}}
We compare \textbf{OQRF} with \textbf{OQRF-nc} to demonstrate that $\widetilde{\Bbeta}_{\tau0}(\cdot)$ still gives a good estimation performance. Here, \textbf{OQRF} denotes the proposed estimator, while \textbf{OQRF-nc} refers to its counterpart that estimates $\Bbeta^{\star}_\tau(\mathbf{x}_0)$ using the non-smoothed quantile regression approach (9) of the main article.

As shown in Table~\ref{OQRF and OQRF_nc}, the numerical performance of \textbf{OQRF} and \textbf{OQRF-nc} is nearly identical, although the convergence rate of $\widetilde{\Bbeta}_{\tau0}(\Bx_0)$ is slightly slower. This confirms that whether we employ the convolution quantile loss function or the original quantile loss function for nuisance parameter estimation has negligible effect on the estimation of treatment effect.

\begin{table}\label{OQRF and OQRF_nc}
\tiny
\centering
\caption{Bias and root-MISE comparison across \textbf{OQRF} and \textbf{OQRF-nc}.}
\renewcommand{\arraystretch}{0.9}
\resizebox{\linewidth}{!}{
\begin{tabular}{ll|cc|cc}
\toprule
\multicolumn{2}{c}{}&\multicolumn{2}{|c|}{\textbf{Bias}}& \multicolumn{2}{c}{\textbf{Root-MISE}}\\
\midrule
&  & OQRF & OQRF-nc & OQRF & OQRF-nc  \\
\midrule
\multicolumn{6}{c}{Setting 1}\\
\midrule
\multirow{3}{*}{p=201} 
& Normal & $\bm{0.06}$ & $\bm{0.06}$ & $\bm{0.08}$ & $\bm{0.08}$\\
& $t_3$   & $\bm{0.07}$ & $\bm{0.07}$ &  $\bm{0.09}$ & $\bm{0.09}$\\
& Cauchy & $\bm{0.10}$ & $\bm{0.10}$  & $\bm{0.13}$ & $\bm{0.13}$\\
\midrule

\multirow{3}{*}{p=501} 
& Normal & $\bm{0.06}$ & $\bm{0.06}$ & $\bm{0.09}$ & $\bm{0.09}$ \\
& $t_3$   & $\bm{0.07}$ & $\bm{0.07}$ & 0.09 & $\bm{0.08}$ \\
& Cauchy  & $\bm{0.10}$ & $\bm{0.10}$ & $\bm{0.13}$ & $\bm{0.13}$ \\
\midrule
\multicolumn{6}{c}{Setting 2}\\
\midrule
\multirow{3}{*}{p=201} 
& Normal  & $\bm{0.07}$ & $\bm{0.07}$ & $\bm{0.09}$ & $\bm{0.09}$ \\
& $t_3$   & 0.09 & $\bm{0.08}$ &  $\bm{0.11}$ & $\bm{0.11}$ \\
& Cauchy  & $\bm{0.12}$ & $\bm{0.12}$ & 0.16  & $\bm{0.15}$ \\
\midrule

\multirow{3}{*}{p=501} 
& Normal  & $\bm{0.07}$ & $\bm{0.07}$ & $\bm{0.09}$ & $\bm{0.09}$\\
& $t_3$  & 0.09 & $\bm{0.08}$ & $\bm{0.11}$ &$\bm{0.11}$ \\
& Cauchy & 0.13 & $\bm{0.12}$ & 0.16 & $\bm{0.15}$ \\
\midrule
\multicolumn{6}{c}{Setting 3}\\
\midrule
\multirow{3}{*}{p=201} 
& Normal  & $\bm{0.07}$ & $\bm{0.07}$  &  $\bm{0.10}$ & 0.11\\
& $t_3$   & $\bm{0.08}$ & 0.09  &  $\bm{0.11}$ & $\bm{0.11}$ \\
& Cauchy  &  $\bm{0.11}$ & $\bm{0.11}$  & 0.15 & $\bm{0.14}$\\
\midrule

\multirow{3}{*}{p=501} 
& Normal  & $\bm{0.07}$ & $\bm{0.07}$ & 0.09 & $\bm{0.09}$ \\
& $t_3$ & $\bm{0.08}$ & $\bm{0.08}$ & $\bm{0.10}$ & $\bm{0.10}$ \\
& Cauchy  & 0.12 & $\bm{0.11}$ &0.15 & $\bm{0.14}$ \\
\bottomrule
\end{tabular}}
\end{table}

\subsection{Cross-sectional Setting}
In this section, we present numerical results under additional settings. While our primary focus is on longitudinal data, we also demonstrate that our method can be applied to cross-sectional data. Cross-sectional data can be viewed as a special case of longitudinal data where each subject is observed only once (i.e., the number of observations per subject is $1$). Specifically, the data is generated from
\begin{align*}
Q_\tau\left(Y_i \mid \mathbf{T}_i, \mathbf{W}_i, \mathbf{X}_i\right) &= \boldsymbol{\theta}_\tau(\mathbf{X}_i)^{\top} \mathbf{T}_i + \boldsymbol{\beta}_\tau(\mathbf{X}_i)^{\top} \mathbf{W}_i, \\
\mathbf{T}_i &= \mathbf{L}(\mathbf{X}_i)^{\top} \mathbf{W}_i + \mathbf{e}_i.
\end{align*}

We conduct simulations under the same three settings for $\Btheta(\BX)$ as in Section 4 of the main text. The methods evaluated here follow those presented in Section 4, and their performance results are shown in Table~\ref{Cross-sectional}, which is consistent with the conclusions reported therein.

\begin{sidewaystable}\label{Cross-sectional}
\centering
\caption{Bias and root-MISE comparison across methods.}
\renewcommand{\arraystretch}{1.2}
\resizebox{\linewidth}{!}{
\begin{tabular}{ll|ccccc|ccccc}
\toprule
\multicolumn{2}{c}{}&\multicolumn{5}{|c|}{\textbf{Bias}}& \multicolumn{5}{c}{\textbf{Root-MISE}}\\
\midrule
&  & OQRF & OQRF-nc & ORF & DML-LA & DML-RF& OQRF & OQRF-nc & ORF & DML-LA & DML-RF \\
\midrule
\multicolumn{12}{c}{Setting 1}\\
\midrule
\multirow{3}{*}{p=201} 
& Normal & 0.09 & $\bm{0.08}$ & 0.10 & 0.15 & 0.30 & $\bm{0.11}$ & $\bm{0.11}$ & 0.13 & 0.20 & 0.36\\
& $t_3$   & $\bm{0.10}$ & $\bm{0.10}$ & 0.16 & 0.16 & 0.30 &  $\bm{0.13}$ & $\bm{0.13}$ & 0.20 & 0.20 & 0.35\\
& Cauchy & 0.16 & $\bm{0.15}$ & 18.33 & 14.33 & 12.47 & 0.21 & $\bm{0.20}$ & 47.68 & 18.32 & 14.87 \\
\midrule

\multirow{3}{*}{p=501} 
& Normal & $\bm{0.08}$ & $\bm{0.08}$ & 0.11 & 0.18 & 0.29 & 0.11 & $\bm{0.10}$ & 0.13 & 0.23 & 0.35 \\
& $t_3$   & $\bm{0.10}$ & $\bm{0.10}$ & 0.17  & 0.19 & 0.30 & $\bm{0.13}$ & $\bm{0.13}$ & 0.21 & 0.24 & 0.35\\
& Cauchy  & $\bm{0.15}$ & $\bm{0.15}$ & 4.28 & 6.31 & 3.50 & 0.20 & $\bm{0.19}$ & 6.99 & 8.25 & 4.56\\
\midrule
\multicolumn{12}{c}{Setting 2}\\
\midrule
\multirow{3}{*}{p=201} 
& Normal  & $\bm{0.10}$ & $\bm{0.10}$ & $\bm{0.10}$ & 0.18 & 0.21 & 0.13 & $\bm{0.12}$ & 0.13 & 0.22 & 0.26\\
& $t_3$   & 0.12 & $\bm{0.11}$& 0.16 & 0.22 & 0.20 & $\bm{0.15}$ & $\bm{0.15}$ & 0.19 & 0.27 & 0.26 \\
& Cauchy  & 0.19 & $\bm{0.18}$ & 12.34 & 14.44 & 10.13 &  0.24  & $\bm{0.23}$ & 28.30 & 17.52 & 12.96\\
\midrule

\multirow{3}{*}{p=501} 
& Normal  & 0.10 & $\bm{0.09}$ & 0.11 & 0.14 & 0.21 & 0.13 & $\bm{0.12}$ & 0.13 & 0.18 & 0.26\\
& $t_3$  & $\bm{0.12}$ & $\bm{0.12}$ & 0.17 & 0.15 & 0.21 & $\bm{0.15}$ &$\bm{0.15}$ & 0.21 & 0.19 & 0.26\\
& Cauchy & 0.19 & $\bm{0.18}$ & 3.78 & 2.37 & 3.40   & 0.24 & $\bm{0.23}$ & 6.65 & 2.88 & 4.15\\
\midrule
\multicolumn{12}{c}{Setting 3}\\
\midrule
\multirow{3}{*}{p=201} 
& Normal  & $\bm{0.11}$ & $\bm{0.11}$ & 0.27 & 0.20 & 0.34 &  0.15 & $\bm{0.14}$  & 0.34 & 0.26 & 0.44\\
& $t_3$   & $\bm{0.13}$ & $\bm{0.13}$ & 0.31 & 0.21 & 0.34  &  $\bm{0.17}$ & 0.18 & 0.39 & 0.28 & 0.45\\
& Cauchy  &  $\bm{0.18}$ & 0.19 & 7.99 & 8.34 & 7.74 &$\bm{0.27}$ & 0.34 & 16.01 & 12.53 & 10.58\\
\midrule

\multirow{3}{*}{p=501} 
& Normal  & 0.11 & $\bm{0.10}$ & 0.29 & 0.23 & 0.34 & 0.15 & $\bm{0.13}$ & 0.35 & 0.32 & 0.45\\
& $t_3$ & 0.13 & $\bm{0.12}$ & 0.33 & 0.25 & 0.35  & $\bm{0.16}$ & $\bm{0.16}$ & 0.40 & 0.33 & 0.46\\
& Cauchy  & 0.19 & $\bm{0.18}$ & 5.69 & 5.66 & 4.00 & $\bm{0.24}$ & $\bm{0.24}$ & 9.89 & 8.65 & 6.03\\
\bottomrule
\end{tabular}}
\end{sidewaystable}

\section{Proof of the Neyman Orthogonality in (4) of the Main Text}
By model assumptions, $\Pr(\varepsilon\le0\mid \BX)=\tau$, and because $\BL^{\star}(\BX)$ is the conditional least-squares coefficient of $\BT$ on $\BW$, each component of the residual $\Be = \BT-\BL^{\star}(\BX)^\top\BW$ satisfies
\[
\mathbb{E}[\,\BW\,\Be\mid \BX] = 0.
\]
This orthogonality comes \emph{for free} from the definition of $\BL^{\star}(\BX)$, so no additional assumption is needed.

For any perturbations $\mathbf{g}_1(\cdot),\mathbf{g}_2(\cdot)$, set
\[
\Bbeta_r = \Bbeta_\tau^{\star} + r\,\mathbf{g}_1,
\quad
\BL_r    = \BL^{\star} + r\,\mathbf{g}_2.
\]
Then the perturbed score is
\begin{align*}
\Bpsi_r &= \varphi_\tau\bigl(Y - \Btheta^{\star\top} \BT - \Bbeta_r^\top \BW\bigr)\;\bigl(\BT - \BL_r^\top \BW\bigr) \\
       &= \varphi_\tau\bigl(\varepsilon - r\,\mathbf{g}_1(\BX)^\top \BW\bigr)\,\bigl(\Be - r\,\mathbf{g}_2(\BX)^\top \BW\bigr).
\end{align*}
Differentiating under expectation and using $\partial_{\varepsilon}\mathbb{E}\left[\varphi_\tau(\varepsilon)\right]=\delta(\varepsilon)$ gives
\[
\frac{d}{dr}\mathbb{E}[\Bpsi_r]\Bigm|_{r=0}
= -\,\mathbb{E}[\,\mathbf{g}_1(\BX)^\top \BW\,\Be\,\delta(\varepsilon)]
   -\,\mathbb{E}[\varphi_\tau(\varepsilon)\,\mathbf{g}_2(\BX)^\top \BW].
\]
We show each term vanishes:
\begin{enumerate}
  \item $\displaystyle\mathbb{E}[\varphi_\tau(\varepsilon)\,\mathbf{g}_2(\BX)^\top \BW]
    = \mathbb{E}\bigl[\mathbf{g}_2(\BX)^\top\mathbb{E}[\varphi_\tau(\varepsilon)\,\BW\mid \BX]\bigr]=\bm{0},$
    since $\mathbb{E}[\varphi_\tau(\varepsilon)\mid \BX]=0$ and $\mathbb{E}[\varphi_\tau(\varepsilon)\,\BW\mid \BX]=\bm{0}$ by quantile regression theory.
  \item $\displaystyle\mathbb{E}[\,\mathbf{g}_1(\BX)^\top \BW\,\Be\,\delta(\varepsilon)]= \mathbb{E}\bigl[\, f_{\varepsilon\mid \BX}(0)\,\mathbf{g}_2(\BX)^\top\,\mathbb{E}[\BW\,\mathbf{e}\mid \BX]\bigr]=\bm{0},
$
    where $\mathbb{E}[\BW\,\Be\mid \BX]=\bm{0}$ by the projection property.
\end{enumerate}
Hence the Gateaux derivative vanishes, establishing Neyman‐orthogonality.  Consequently, small first‐stage errors in $(\Bbeta,\BL)$ affect the estimator of $\Btheta$ only at higher order, enabling a faster convergence rate and valid inference for the parameter of interest.

\section{Proof of Main Results}
\subsection{Proof of Results in Section \ref{Nuisance-property}}
\begin{lemma}{\textbf{(Restricted Strong Convexity)}}\label{lemmassum:design_matrix}
     Suppose the conditions in Theorem~\ref{thm_conv} are satisfied, then with probability $1-\gamma$, 
     \begin{equation}\label{eq25}
     \begin{aligned}
         &\quad\frac{\left\langle  \nabla\widehat{Q}_{\tau h}(\Bzeta)-\nabla\widehat{Q}_{\tau h}(\Bzeta^{\star}_\tau(\Bx_0)),\Bzeta-\Bzeta^{\star}_\tau(\Bx_0)\right\rangle}{\left\|\BSigma^{1/2}\left\{\Bzeta-\Bzeta^{\star}_\tau(\Bx_0)\right\}\right\|^2}\\
         &\geq \kappa_l\left\lbrace\frac{9\underline{f}\left(1-c_0e^{-1}\right)}{32}-\sqrt\frac{s\log(1/\gamma)}{nh^2}-Ls^{-\frac{1}{2\omega d}}/h\right\rbrace,
     \end{aligned}
     \end{equation}
     for any $\Bzeta$ satisfies $\left\|\BSigma^{1/2}\left\{\Bzeta-\Bzeta^{\star}_\tau(\Bx_0)\right\}\right\|\leq r$, where $r\leq h/(20v_0^2)$, with $\underline{f}$ defined in Assumption~\ref{assum:density}, $c_0$ defined in Assumption \ref{assum:design_subgaussian} and $\omega$ defined in Assumption~\ref{sparsity level}.
\end{lemma}
\begin{proof}
    The proof is similar to Proposition 4.2 in \cite{tan2022high}. Define the symmetric Bregman divergence between $\Bzeta$ and $\Bzeta^{\star}_\tau(\Bx_0)$
    $$B(\Bzeta)=\left\langle\nabla\widehat{Q}_{\tau h}(\Bzeta)-\nabla\widehat{Q}_{\tau h}(\Bzeta^{\star}_\tau(\Bx_0)),\Bzeta-\Bzeta^{\star}_\tau(\Bx_0)\right\rangle$$
    and the event
    \begin{align*}
        E_{ij}=&\left\{\left|\varepsilon_{ij}\right|\leq\frac{h}{4}\right\}\cap\left\{\frac{\left|\left\lbrace\Bzeta-\Bzeta^{\star}_\tau(\Bx_0)\right\rbrace^{\top}\BD_{ij}\right|}{\left\|\BSigma^{1/2}\left\{\Bzeta-\Bzeta^{\star}_\tau(\Bx_0)\right\}\right\|}\leq\frac{h}{2r}\right\}\\
        &\cap\left\{\left|\left\lbrace\Bzeta^{\star}_\tau(\Bx_0)-\Bzeta^{\star}_\tau(\BX_i)\right\rbrace^{\top}\BD_{ij}\right|\leq C_1s^{-\frac{1}{2\omega d}}\text{ for any $i$ satisfies $\alpha_i>0$}\right\}.
    \end{align*}
    To establish the desired result, we proceed in two main steps. We first derive a tractable lower bound for $\frac{B(\Bzeta)}{\left\|\BSigma^{1/2}\left\{\Bzeta-\Bzeta^{\star}_\tau(\Bx_0)\right\}\right\|^2}$, denoted as $\underline{B}(\Bzeta)$ as in (\ref{B_lowerbound}), which provides a convenient way to control the curvature of the objective function around the true parameter. We then provide a uniform lower bound for $\underline{B}(\Bzeta)$.

    \textbf{Derive a tractable lower bound function for $\frac{B(\Bzeta)}{\left\|\BSigma^{1/2}\left\{\Bzeta-\Bzeta^{\star}_\tau(\Bx_0)\right\}\right\|^2}$.} For any $i$ satisfying $\alpha_i>0$, conditioned on the event $E_{ij}$ and combine with the assumption on $h$, we have
    \begin{equation}
        \begin{aligned}
            \left|\frac{\Bzeta^{\top}\BD_{ij}-Y_{ij}}{h}\right|&\leq\left|\frac{\left\lbrace\Bzeta-\Bzeta^{\star}_\tau(\Bx_0)\right\rbrace^{\top}\BD_{ij}}{h}\right|+ \left|\frac{\left\lbrace\Bzeta^{\star}_\tau(\Bx_0)-\Bzeta^{\star}_\tau(\BX_i)\right\rbrace^{\top}\BD_{ij}}{h}\right|+\left|\frac{\varepsilon_{ij}}{h}\right|\\
            &\leq \frac{\left\|\BSigma^{1/2}\left\{\Bzeta-\Bzeta^{\star}_\tau(\Bx_0)\right\}\right\|}{2r}+\frac{C_1s^{-\frac{1}{2\omega d}}}{h}+\left|\frac{\varepsilon_{ij}}{h}\right|\\
            &\leq\frac{1}{2}+\frac{1}{4}+\frac{1}{4}=1,
        \end{aligned}
        \nonumber
    \end{equation}
where the second inequality follows from the assumption on $\Bzeta$ and Proposition~\ref{thm:shrinkage}. Furthermore, $\left|\frac{\Bzeta^{\star}_\tau(\Bx_0)^{\top}\BD_{ij}-Y_{ij}}{h}\right|\leq \left|\frac{\left\lbrace\Bzeta^{\star}_\tau(\Bx_0)-\Bzeta^{\star}_\tau(\BX_i)\right\rbrace^{\top}\BD_{ij}}{h}\right|+\left|\frac{\varepsilon_{ij}}{h}\right|<1$. Then we have
    \begin{equation}\label{S2}
    \begin{aligned}            B(\Bzeta)&=\sum_{i=1}^n\alpha_i(\Bx_0)\sum_{j=1}^{m_i}\frac{1}{m_i}\left\{\bar{K}\left(\frac{\Bzeta^{\top}\BD_{ij}-Y_{ij}}{h}\right)-\bar{K}\left(\frac{\Bzeta^{\star}_\tau(\Bx_0)^{\top}\BD_{ij}-Y_{ij}}{h}\right)\right\}\\
            &\quad\cdot\left\lbrace\Bzeta-\Bzeta^{\star}_\tau(\Bx_0)\right\rbrace^{\top}\BD_{ij}\\
            &\geq \sum_{i=1}^n\alpha_i(\Bx_0)\frac{\kappa_l}{h}\sum_{j=1}^{m_i}\frac{1}{m_i}\left[\left\lbrace\Bzeta-\Bzeta^{\star}_\tau(\Bx_0)\right\rbrace^{\top}\BD_{ij}\right]^2\cdot I_{E_{ij}}.
    \end{aligned}
    \end{equation}
To further derive the lower bound of the right side of \eqref{S2}, which contains an indicator function $I_{E_{ij}}$, we define the function
    \begin{equation}
    \phi_R(u)=\left\{
	\begin{array}{cl}
		u^2 &  0\leq |u|\leq R/2,\\
		\left\lbrace u-R\text{sign}(u)\right\rbrace^2 &  R/2<|u|\leq R, \\
		0& |u|> R, \\
	\end{array} \right.
	\nonumber
    \end{equation}
where $R$ is a positive constant. The function $\phi_R(u)$ satisfies 
    \begin{equation}\label{phi property}
    u^2I\left(|u|\leq R/2\right)\leq\phi_R(u)\leq u^2I\left((|u|\leq R\right).
    \end{equation}
     The left side of \eqref{eq25} can be lower bounded by
     \begin{equation}\label{B_lowerbound}
     \begin{aligned}
         &\quad\frac{B(\Bzeta)}{\left\|\BSigma^{1/2}\left\{\Bzeta-\Bzeta^{\star}_\tau(\Bx_0)\right\}\right\|^2}\\
         &\geq\frac{\kappa_l}{h}\sum_{i=1}^n\alpha_i(\Bx_0)\sum_{j=1}^{m_i}\frac{1}{m_i}\underbrace{\phi_{h/(2r)}\left(\frac{\left\lbrace\Bzeta-\Bzeta^{\star}_\tau(\Bx_0)\right\rbrace^{\top}\BD_{ij}}{\left\|\BSigma^{1/2}\left\{\Bzeta-\Bzeta^{\star}_\tau(\Bx_0)\right\}\right\|}\right)\cdot\mathcal{A}_{ij}}_{\mathcal{C}_{ij}}\cdot\mathcal{B}_{ij},
     \end{aligned}
     \end{equation}
 where $\mathcal{A}_{ij}=I\left(\left|\left\lbrace\Bzeta^{\star}_\tau(\Bx_0)-\Bzeta^{\star}_\tau(\BX_i)\right\rbrace^{\top}\BD_{ij}\right|\leq C_1s^{-\frac{1}{2\omega p_x}}\right)$ and $\mathcal{B}_{ij}=I\left(\left|\varepsilon_{ij}\right|\leq\frac{h}{4}\right)$. 
 Denote $\underline{B}(\Bzeta)=\frac{\kappa_l}{h}\sum_{i=1}^n\alpha_i(\Bx_0)\sum_{j=1}^{m_i}\frac{1}{m_i}\phi_{h/(2r)}\left(\frac{\left\lbrace\Bzeta-\Bzeta^{\star}_\tau(\Bx_0)\right\rbrace^{\top}\BD_{ij}}{\left\|\BSigma^{1/2}\left\{\Bzeta-\Bzeta^{\star}_\tau(\Bx_0)\right\}\right\|}\right)\cdot\mathcal{A}_{ij}\mathcal{B}_{ij}$, which is a lower bound function for $\frac{B(\Bzeta)}{\left\|\BSigma^{1/2}\left\{\Bzeta-\Bzeta^{\star}_\tau(\Bx_0)\right\}\right\|^2}$. 
 
 \textbf{Then we aim to get the lower bound of $\underline{B}(\Bzeta)$.} To accomplish this, we bound $\mathbb{E}\left[\underline{B}(\Bzeta)\mid\Bx_0\right]$ and $\left|\underline{B}(\Bzeta)-\mathbb{E}\left[\underline{B}(\Bzeta)\mid\Bx_0\right]\right|$ respectively. For the term $\mathbb{E}\left[\underline{B}(\Bzeta)\mid\Bx_0\right]$: since $\mathcal{C}_{ij}$ is independent of $\mathcal{B}_{ij}$, we get the lower bound for $\mathbb{E}\left[\mathcal{B}_{ij}\mid \Bx_0\right]$ and $\mathbb{E}\left[\mathcal{C}_{ij}\mid \Bx_0\right]$ separately. With Assumption~\ref{assum:density},
 \begin{equation}\label{eq26}
         \left|\mathbb{E}\left[\mathcal{B}_{ij}\right]-\frac{h}{2}f_\varepsilon(0)\right|\leq\int_{-\frac{h}{4}}^{\frac{h}{4}}\left|f_\varepsilon(t)-f_\varepsilon(0)\right|dt\leq\frac{h^2\bar{f}'}{8}.
 \end{equation}
 Then $\mathbb{E}\left[\mathcal{B}_{ij}\right]$ can be lower bounded by 
 \begin{equation}\label{chi lower bound}
         \quad\mathbb{E}\left[\mathcal{B}_{ij}\right]\geq \frac{h}{2}f_\varepsilon(0)-\frac{h^2\bar{f}'}{8}\geq \frac{h \underline{f}}{2}-\frac{h^2\bar{f}'}{8}\geq \frac{3h \underline{f}}{8},
 \end{equation}
where the last inequality follows from the condition of bandwidth. We then proceed to study the lower bound of $\mathbb{E}\left[\mathcal{C}_{ij} \mid \Bx_0\right]$. Denote $\Bdelta_0=\Bzeta-\Bzeta^{\star}_\tau(\Bx_0)$, $\Bdelta_i=\Bzeta^{\star}_\tau(\Bx_0)-\Bzeta^{\star}_\tau(\BX_i)$ and $\iota_{ij}\left(\Bdelta\right)=\Bdelta^{\top}\BD_{ij}/\left\|\BSigma^{1/2}\Bdelta(\Bx_0)\right\|$. With the second part of Assumption~\ref{assum:design_subgaussian}, two random variales $\phi_{h/(2r)}\left(\frac{\left\lbrace\Bzeta-\Bzeta^{\star}_\tau(\Bx_0)\right\rbrace^{\top}\BD_{ij}}{\left\|\BSigma^{1/2}\left\{\Bzeta-\Bzeta^{\star}_\tau(\Bx_0)\right\}\right\|}\right)$ and $\mathcal{A}_{ij}$ are non-negatively correlated, then we have
 \begin{equation}
     \begin{aligned}
         &\quad\mathbb{E}\left[\phi_{h/(2r)}\left(\frac{\left\lbrace\Bzeta-\Bzeta^{\star}_\tau(\Bx_0)\right\rbrace^{\top}\BD_{ij}}{\left\|\BSigma^{1/2}\left\{\Bzeta-\Bzeta^{\star}_\tau(\Bx_0)\right\}\right\|}\right)\cdot\mathcal{A}_{ij}\mid\Bx_0\right]\\
         &\geq\mathbb{E}\left[\phi_{h/(2r)}\left(\iota_{ij}\left(\Bdelta_0\right)\right)\mid\Bx_0\right]\cdot \mathbb{E}\left[\mathcal{A}_{ij}\mid\Bx_0\right]\\
         &\geq\mathbb{E}\left[\left\lbrace\iota_{ij}\left(\Bdelta(\Bx_0)\right)\right\rbrace^2I\left(\left|\iota_{ij}\left(\Bdelta_0\right)\right|\leq h/(4r)\right)\mid\Bx_0\right]\cdot \mathbb{E}\left[\mathcal{A}_{ij}\mid\Bx_0\right].
     \end{aligned}
     \nonumber
 \end{equation}
 Note that $\mathbb{E}\left[\iota_{ij}^2\left(\Bdelta_0\right)\mid\Bx_0\right]=1$, then
    \begin{equation*}
        \begin{aligned}
            &\quad\mathbb{E}\left[\left\lbrace\iota_{ij}\left(\Bdelta(\Bx_0)\right)\right\rbrace^2I\left(\left|\iota_{ij}\left(\Bdelta_0\right)\right|\leq h/(4r)\right)\mid\Bx_0\right]\\
            &\geq1-\mathbb{E}\left[\left\lbrace\iota_{ij}\left(\Bdelta(\Bx_0)\right)\right\rbrace^2I\left(\left|\iota_{ij}\left(\Bdelta_0\right)\right|\geq h/(4r)\right)\mid\Bx_0\right].
        \end{aligned}
    \end{equation*}
With the sub-Gaussian condition of $\BD_{ij}$ and the condition $r\leq h/(20v_0^2)$, $$\mathbb{E}\left[\iota_{ij}^2\left(\Bdelta_0\right)\cdot I\left\{|\iota_{ij}\left(\Bdelta_0\right)|>\frac{h}{4r}\right\}\mid\Bx_0\right]<\frac{1}{4},$$
which follows directly from the proof of Proposition 4.2 in \cite{tan2022high}. For the term $\mathbb{E}\left[\mathcal{A}_{ij}\mid\Bx_0\right]$, $\mathbb{E}\left[\mathcal{A}_{ij}\mid\Bx_0\right]=\mathbb{P}\left[\left|\left\lbrace\Bzeta^{\star}_\tau(\Bx_0)-\Bzeta^{\star}_\tau(\BX_i)\right\rbrace^{\top}\BD_{ij}\right|\leq C_1s^{-\frac{1}{2\omega p_x}}\right]=1-c_0e^{-1}$, where the last equality follows from the first part in Assumption~\eqref{assum:design_subgaussian}. Therefore $\mathbb{E}\left[\underline{B}(\Bzeta)\mid\Bx_0\right]$ can be lower bounded by:
 \begin{equation}\label{eq27}
\mathbb{E}\left[\underline{B}(\Bzeta)\mid\Bx_0\right]\geq\frac{9\kappa_l\underline{f}\left(1-c_0e^{-1}\right)}{32}.
 \end{equation}
Next we bound  $\left|\underline{B}(\Bzeta)-\mathbb{E}\left[\underline{B}(\Bzeta)\mid\Bx_0\right]\right|$. By the U-statistics Hoeffding inequality and Proposition~\ref{thm:shrinkage}, we have, with probability $1-\gamma$,
 \begin{equation}\label{eq28}
     \begin{aligned}
         &\quad\left|\underline{B}(\Bzeta)-\mathbb{E}\left[\underline{B}(\Bzeta)\mid\Bx_0\right]\right|\\
         &\leq\left|\underline{B}(\Bzeta)-\frac{\kappa_l}{h}\sum_{i=1}^n\alpha_i(\Bx_0)\mathbb{E}\left[\phi_{h/(2r)}\left(\frac{\left\lbrace\Bzeta-\Bzeta^{\star}_\tau(\Bx_0)\right\rbrace^{\top}\BD_{ij}}{\left\|\BSigma^{1/2}\left\{\Bzeta-\Bzeta^{\star}_\tau(\Bx_0)\right\}\right\|}\right)\cdot\mathcal{A}_{ij}\mathcal{B}_{ij}\mid\BX_i\right]\right|+\\
          &\quad\left|\frac{\kappa_l}{h}\sum_{i=1}^n\alpha_i(\Bx_0)\mathbb{E}\left[\phi_{h/(2r)}\left(\frac{\left\lbrace\Bzeta-\Bzeta^{\star}_\tau(\Bx_0)\right\rbrace^{\top}\BD_{ij}}{\left\|\BSigma^{1/2}\left\{\Bzeta-\Bzeta^{\star}_\tau(\Bx_0)\right\}\right\|}\right)\cdot\mathcal{A}_{ij}\mathcal{B}_{ij}\mid\BX_i\right]-\mathbb{E}\left[\underline{B}(\Bzeta)\mid\Bx_0\right]\right|\\
         &\leq \frac{\kappa_l}{h}\left(\sqrt\frac{s\log(1/\gamma)}{n}+Ls^{-\frac{1}{2\omega p_x}}\right).
     \end{aligned}
 \end{equation}
Combine \eqref{eq27} with \eqref{eq28}, 
\begin{equation}
    \underline{B}(\Bzeta)\geq \frac{9\kappa_l\underline{f}\left(1-c_0e^{-1}\right)}{32}-\frac{\kappa_l}{h}\left(\sqrt\frac{s\log(1/\gamma)}{n}+Ls^{-\frac{1}{2\omega p_x}}\right).
\end{equation}
Thus the conclusion~\eqref{eq25} can be proved.
\end{proof}

\noindent\textbf{Proof of Theorem~\ref{thm_conv}:} 
\begin{proof}
Denote $\widetilde{\Bdelta}(\Bx_0)=\widetilde{\Bzeta}_{\tau h}(\Bx_0)-\Bzeta^{\star}_\tau(\Bx_0)$. To derive the $\ell_2$-error bound of $\widetilde{\Bzeta}_{\tau h}(\Bx_0)$, we establish both lower and upper bounds for the intermediate variable $B(\widetilde{\Bzeta}_{\tau h}(\Bx_0))$ defined in (\ref{S2}), and use them to control the deviation $\left\|\widetilde{\Bzeta}_{\tau h}(\Bx_0) - \Bzeta_\tau^{\star}(\Bx_0)\right\|_2$. Specifically, we show that the upper bound of $B(\widetilde{\Bzeta}_{\tau h}(\Bx_0))$ can be expressed as a linear function of $\left\|\widetilde{\Bdelta}(\Bx_0)\right\|$, while the lower bound can be expressed as a quadratic function of $\left\|\widetilde{\Bdelta}(\Bx_0)\right\|$. Combining these two results yields an inequality involving $\left\|\widetilde{\Bdelta}(\Bx_0)\right\|$, from which the desired $\ell_2$-error bound is derived.

\textbf{First, we get the upper bound of $B(\widetilde{\Bzeta}_{\tau h}(\Bx_0))$ defined in (\ref{S2}).} By the optimality of $\widetilde{\Bzeta}_{\tau h}(\Bx_0)$, there exists a subgradient $\widehat{g}\in\partial\left\|\widetilde{\Bzeta}_{\tau h}(\Bx_0)\right\|_1$  such that $\nabla\widehat{Q}_{\tau h}(\widetilde{\Bzeta}_{\tau h}(\Bx_0))+ \frac{\lambda_2}{n_{rf}}\widehat{g}=0$. Note that
 \begin{equation}\label{optimality of zeta}
 \begin{aligned}
        &\quad\left\langle\nabla\widehat{Q}_{\tau h}(\widetilde{\Bzeta}_{\tau h}(\Bx_0))-\nabla\widehat{Q}_{\tau h}(\Bzeta^{\star}_\tau(\Bx_0)),\widetilde{\Bzeta}_{\tau h}(\Bx_0)-\Bzeta^{\star}_\tau(\Bx_0)\right\rangle\\
         &=\frac{\lambda_2}{n_{rf}} \left\langle\widehat{g},\Bzeta^{\star}_\tau(\Bx_0)-\widetilde{\Bzeta}_{\tau h}(\Bx_0)\right\rangle+\left\langle\nabla\widehat{Q}_{\tau h}(\Bzeta^{\star}_\tau(\Bx_0)),\Bzeta^{\star}_\tau(\Bx_0)-\widetilde{\Bzeta}_{\tau h}(\Bx_0)\right\rangle.\\
 \end{aligned}
 \end{equation}
 We need to obtain the upper bound of the gradient $\left\|\nabla\widehat{Q}_{\tau h}(\Bzeta^{\star}_\tau(\Bx_0))\right\|_\infty$. Denote the sub-Gaussian norm of $\BD_{ij}$ as $C_3$, then with probability $1-2\gamma$,
\begin{equation}
	\begin{aligned}
		&\quad\left\|\nabla\widehat{Q}_{\tau h}(\Bzeta^{\star}_\tau(\Bx_0))\right\| _\infty\\
        &\leq	\left\|\sum_{i=1}^n \alpha_i(\Bx_0)\sum_{j=1}^{m_i}\frac{1}{m_i}\mathbb{E}\left[ \left\{\bar{K}\left(\frac{\Bzeta^{\star}_\tau(\Bx_0)^{\top}\BD_{ij}}{h}\right)-\tau\right\}\BD_{ij}\mid\BX_i\right] \right\| _\infty\\
        &\quad+C_3\sqrt{\frac{s\log\left(\left(p_t+p_w \right)/\gamma  \right) }{n}}\\
	 &\leq \left\|\sum_{i=1}^n\alpha_i(\Bx_0)\mathbb{E}\left[ \left\{F_{Y_{ij}\mid\BD_{ij}}\left(\Bzeta^{\star}_\tau(\Bx_0)^{\top}\BD_{ij}\right)-\tau\right\}\BD_{ij}\mid\BX_i\right] \right\| _\infty+C_2h^2\\
     &\quad+ C_3\sqrt{\frac{s\log\left(\left(p_t+p_w \right)/\gamma\right)}{n}}\\
        &=\left\|\sum_{i=1}^n\alpha_i(\Bx_0)\mathbb{E}\left[ \left\{F_{Y_{ij}\mid\BD_{ij}}\left(\Bzeta^{\star}_\tau(\Bx_0)^{\top}\BD_{ij}\right)-F_{Y_{ij}|\BD_{ij}}\left(\Bzeta^{\star}_\tau(\BX_i)^{\top}\BD_{ij}\right)\right\}\BD_{ij}\mid\BX_i\right]\right\|_\infty\\
        &\quad+C_2h^2+C_3\sqrt{\frac{s\log\left(\left(p_t+p_w \right)/\gamma\right)}{n}}\\
	&\leq \bar{f}C_1\sqrt{\log\left(c_0/\gamma\right)}s^{-\frac{1}{2\omega p_x}}+C_2h^2+C_3\sqrt{\frac{s\log\left(\left(p_t+p_w \right)/\gamma  \right) }{n}}.\\
	\end{aligned}
 \nonumber
\end{equation}
The first inequality follows from U-statistics Hoeffding inequality, the second inequality follows from Lemma 1 in \citep{fernandes2021smoothing} and the last inequality follows from Proposition~\ref{thm:shrinkage}. So as long as $\frac{\lambda_2}{n_{rf}}\geq \bar{f}C_1\sqrt{\log\left(c_0/\gamma\right)}s^{-\frac{1}{2\omega p_x}}+C_2h^2+\sqrt{\frac{s\log\left(\left(p_t+p_w \right)/\gamma  \right) }{n}} $, there exists a constant $c>1$, $\frac{\lambda_2}{n_{rf}}\geq c\cdot\left\|\frac{\partial}{\partial\Bzeta}\widehat{Q}_{\tau h}\left(\Bzeta^{\star}_\tau(\Bx_0)\right)\right\|_\infty$. Recall that $\widetilde{\Bdelta}(\Bx_0)=\widetilde{\Bzeta}_{\tau h}(\Bx_0)-\Bzeta^{\star}_\tau(\Bx_0)$, combine the upper bound of the gradient $\left\|\nabla\widehat{Q}_{\tau h}(\Bzeta^{\star}_\tau(\Bx_0))\right\|_\infty$ with~\eqref{optimality of zeta}, the upper bound of $B(\widetilde{\Bzeta}_{\tau h}(\Bx_0))$ can be obtained by
\begin{equation}\label{eq29}
\begin{aligned}
 B(\widetilde{\Bzeta}_{\tau h}(\Bx_0))&=\left\langle\nabla\widehat{Q}_{\tau h}(\widetilde{\Bzeta}_{\tau h}(\Bx_0))-\nabla\widehat{Q}_{\tau h}(\Bzeta^{\star}_\tau(\Bx_0)),\widetilde{\Bzeta}_{\tau h}(\Bx_0)-\Bzeta^{\star}_\tau(\Bx_0)\right\rangle\\
    &\leq \frac{\lambda_2}{n_{rf}}\left(\left\|\widetilde{\Bdelta}(\Bx_0)_S\right\|_1-\left\|\widetilde{\Bdelta}(\Bx_0)_{S^C}\right\|_1\right)+\frac{1}{c}\frac{\lambda_2}{n_{rf}}\left\|\widetilde{\Bdelta}(\Bx_0)\right\|_1\\
         &\leq \left(\frac{1}{c}+1\right)\frac{\lambda_2}{n_{rf}}\left\|\widetilde{\Bdelta}(\Bx_0)_S\right\|_1\leq \left(\frac{1}{c}+1\right)\frac{\lambda_2}{n_{rf}}k^{1/2}\left\|\widetilde{\Bdelta}(\Bx_0)\right\|\\
         &\leq\left(\frac{1}{c}+1\right)\frac{\lambda_2}{n_{rf}}\left(\frac{k}{\sigma_{\text{min}}}\right)^{1/2}\left\|\BSigma^{1/2}\widetilde{\Bdelta}(\Bx_0)\right\|.
\end{aligned}
\end{equation}

\textbf{Now we turn to the lower bound of $B(\widetilde{\Bzeta}_{\tau h}(\Bx_0))$.} From Lemma \ref{lemmassum:design_matrix}, we can get the lower bound of $B(\widetilde{\Bzeta}_{\tau h}(\Bx_0))$ when $\left\|\BSigma^{1/2}\left\{\widetilde{\Bzeta}_{\tau h}(\Bx_0)-\Bzeta_\tau^*(\Bx_0)\right\}\right\|\leq r:=h/(20v_0^2)$. We establish the bound $\left\|\BSigma^{1/2}\left\{\widetilde{\Bzeta}_{\tau h}(\Bx_0)-\Bzeta_\tau^*(\Bx_0)\right\}\right\|\leq r$ via a proof by contradiction. Define 
$$b=\sup\left\{u\in[0,1]:\left\|u\BSigma^{1/2}\left\{\widetilde{\Bzeta}_{\tau h}(\Bx_0)-\Bzeta^{\star}_\tau(\Bx_0)\right\}\right\|\leq r\right\}$$ 
and the intermediate estimator
\begin{equation}\label{def:intermediate est}
    \bar{\Bzeta}_\tau(\Bx_0)=(1-b)\Bzeta^{\star}_\tau(\Bx_0)+b\widetilde{\Bzeta}_{\tau h}(\Bx_0),\bar{\Bdelta}(\Bx_0)=\bar{\Bzeta}_{\tau h}(\Bx_0)-\Bzeta^{\star}_\tau(\Bx_0).
\end{equation}
If $\left\|\BSigma^{1/2}\left\{\widetilde{\Bzeta}_{\tau h}(\Bx_0)-\Bzeta^{\star}_\tau(\Bx_0)\right\}\right\|\leq r$, then $b=1$ and $\bar{\Bzeta}_\tau(\Bx_0)=\widetilde{\Bzeta}_{\tau h}(\Bx_0)$; otherwise, if $\left\|\BSigma^{1/2}\left\{\widetilde{\Bzeta}_{\tau h}(\Bx_0)-\Bzeta^{\star}_\tau(\Bx_0)\right\}\right\|>r$, $b\in(0,1)$ and $\left\|\BSigma^{1/2}\left\{\bar{\Bzeta}_\tau(\Bx_0)-\Bzeta_\tau^*(\Bx_0)\right\}\right\|=r$. The intermediate estimator $\bar{\Bzeta}_\tau(\Bx_0)$ is a convex combination of $\Bzeta_\tau^{\star}(\Bx_0)$ and $\widetilde{\Bzeta}_{\tau h}(\Bx_0)$ that lies in the neighborhood of $\Bzeta_\tau^{\star}(\Bx_0)$: it coincides with $\widetilde{\Bzeta}_{\tau h}(\Bx_0)$ when the deviation is within $r$, and otherwise it is truncated so that its distance from $\Bzeta_\tau^*(\Bx_0)$ is exactly $r$. By Lemma F.2 in \cite{fan2018lamm},
 \begin{align*}
     &\quad b\left\langle\nabla\widehat{Q}_{\tau h}(\widetilde{\Bzeta}_{\tau h}(\Bx_0))-\nabla\widehat{Q}_{\tau h}(\Bzeta^{\star}_\tau(\Bx_0)),\widetilde{\Bzeta}_{\tau h}(\Bx_0)-\Bzeta^{\star}_\tau(\Bx_0)\right\rangle\\
     &\geq\left\langle\nabla\widehat{Q}_{\tau h}(\bar{\Bzeta}_{\tau h}(\Bx_0))-\nabla\widehat{Q}_{\tau h}(\Bzeta^{\star}_\tau(\Bx_0)),\bar{\Bzeta}_{\tau h}(\Bx_0)-\Bzeta^{\star}_\tau(\Bx_0)\right\rangle.
 \end{align*}
According to Lemma \ref{lemmassum:design_matrix}, with probability $1-\gamma$,
 \begin{equation}\label{eq30}
 \begin{aligned}
     B(\widetilde{\Bzeta}_{\tau h}(\Bx_0))&=\left\langle\nabla\widehat{Q}_{\tau h}(\widetilde{\Bzeta}_{\tau h}(\Bx_0))-\nabla\widehat{Q}_{\tau h}(\Bzeta^{\star}_\tau(\Bx_0)),\widetilde{\Bzeta}_{\tau h}(\Bx_0)-\Bzeta^{\star}_\tau(\Bx_0)\right\rangle\\
     &\geq\frac{1}{b}\left\langle\nabla\widehat{Q}_{\tau h}(\bar{\Bzeta}_{\tau h}(\Bx_0))-\nabla\widehat{Q}_{\tau h}(\Bzeta^{\star}_\tau(\Bx_0)),\bar{\Bzeta}_{\tau h}(\Bx_0)-\Bzeta^{\star}_\tau(\Bx_0)\right\rangle\\
     &\geq \frac{\widetilde{\kappa}}{b}\left\|\BSigma^{1/2}\bar{\Bdelta}(\Bx_0)\right\|^2.
 \end{aligned}
 \end{equation}
 \textbf{Finally, we employ the method of contradiction to prove that $\bar{\Bzeta}_\tau(\Bx_0)=\widetilde{\Bzeta}_{\tau h}(\Bx_0)$.} If $\left\|{\BSigma}^{1/2}\left\lbrace\widetilde{\Bzeta}_{\tau h}(\Bx_0)-\Bzeta^{\star}_\tau(\Bx_0)\right\rbrace\right\|>r$, combine \eqref{eq29} and \eqref{eq30}, we have
 \begin{equation}
 \begin{aligned}
    \frac{\widetilde{\kappa}}{b}\left\|\BSigma^{1/2}\bar{\Bdelta}(\Bx_0)\right\|^2&\leq \left(\frac{1}{c}+1\right)\left(\frac{k}{\sigma_{\text{min}}}\right)^{1/2}\cdot\frac{\lambda_2}{n_{rf}}\left\|\BSigma^{1/2}\widetilde{\Bdelta}(\Bx_0)\right\|\\
    &\leq\frac{1}{b}\left(\frac{1}{c}+1\right)\left(\frac{k}{\sigma_{\text{min}}}\right)^{1/2}\cdot\frac{\lambda_2}{n_{rf}}\left\|\BSigma^{1/2}\bar{\Bdelta}(\Bx_0)\right\|.
 \end{aligned}
 \end{equation}
Consequently, $\left\|\BSigma^{1/2}\bar{\Bdelta}(\Bx_0)\right\|\leq\frac{1+c}{c\widetilde{\kappa}}\cdot\left(\frac{k}{\sigma_{\text{min}}}\right)^{1/2}\cdot\frac{\lambda_2}{n_{rf}}$ with probability $1-\gamma$. Moreover, with the condition on $\lambda_2$ and $h$, we have $r>\frac{1+c}{c\widetilde{\kappa}}\cdot\left(\frac{k}{\sigma_{\text{min}}}\right)^{1/2}\cdot\frac{\lambda_2}{n_{rf}}$. Then  $\left\|\BSigma^{1/2}\bar{\Bdelta}(\Bx_0)\right\|< r$ and we have $\bar{\Bzeta}_\tau(\Bx_0)=\widetilde{\Bzeta}_{\tau h}(\Bx_0)$ by contradiction. 

Combine \eqref{eq29} and \eqref{eq30}, we have
$$\left(\frac{1}{c}+1\right)\frac{\lambda_2}{n_{rf}}\left(\frac{k}{\sigma_{\text{min}}}\right)^{1/2}\left\|\BSigma^{1/2}\widetilde{\Bdelta}(\Bx_0)\right\|.\geq \kappa\left\|\BSigma^{1/2}\widetilde{\Bdelta}(\Bx_0)\right\|^2.$$
Therefore, the conclusion in Theorem \ref{thm_conv} can be proved.
\end{proof}

Next we prove the error bound of the nuisance parameter $\widetilde{\Bbeta}_{\tau0}(\Bx_0)$, we first define the Jacobian matrix $\BJ_\tau$ as 
$$\BJ_\tau=\mathbb{E}\left[f_{Y_{ij}}\left(\Bzeta^{\star}_{\tau}(\Bx_0)^{\top}\BD_{ij}\right)\BD_{ij}\BD_{ij}^{\top}\mid \Bx_0\right].$$
\begin{lemma}\label{lemma:restricted set}
	Suppose the conditions in Theorem~\ref{thm:beta_nonsmooth} are satisfied, let $e_0>1$ be a constant and $A(e_0):= \{\Bdelta\in\mathbb{R}^{(p_t+p_w)}:\|\Bdelta_{S^c}\|_1\leq e_0\|\Bdelta_{S}\|_1\}$, which coincides with the set defined in Assumption~\ref{assum:design_subgaussian'}. Then for any $\Bdelta\in A(e_0)$, $\Bdelta$ satisfies
	\begin{equation}\label{lemma:restricted set.1}
		\left\| \Bdelta\right\| \leq\left( 1+e_0\sqrt{k/m}\right) \left\|\BJ_\tau^{1/2}\Bdelta\right\| /\left[\underline{f}^{1/2}t_m \right],
	\end{equation}
and
\begin{equation}\label{lemma:restricted set.2}
\begin{aligned}
    &\quad\mathbb{E}\left[\rho_\tau\left(Y_{ij}-\left\lbrace\Bzeta^{\star}_\tau(\Bx_0)+\Bdelta\right\rbrace^{\top}\BD_{ij}\right)\mid\Bx_0 \right]-\mathbb{E}\left[\rho_\tau\left(Y_{ij}-\Bzeta^{\star}_\tau(\Bx_0)^{\top}\BD_{ij}\right)|\Bx_0 \right]\\
    &\geq\left(\left\|\BJ_\tau^{1/2}\Bdelta\right\| ^2/4 \right)\wedge \left(t\left\|\BJ_\tau^{1/2}\Bdelta \right\|  \right) .
\end{aligned}
\end{equation}
\end{lemma}
The proof of Lemma~\ref{lemma:restricted set} is similar to the proof of Lemma 4 in \cite{belloni2011ℓ}.

~\\

\noindent\textbf{Proof of Theorem~\ref{thm:beta_nonsmooth}:} 
\begin{proof}
We first show that the estimator’s deviation $\widetilde{\Bdelta}(\Bx_0)=\widetilde{\Bzeta}_{\tau0}(\Bx_0)-\Bzeta^{\star}_\tau(\Bx_0)$ lies in a restricted set $ A(e_0) := \{\Bdelta\in\mathbb{R}^{(p_t+p_w)}:\|\Bdelta_{S^c}\|_1\leq e_0\|\Bdelta_{S}\|_1\}$. Next, we derive an upper bound for $\widehat{Q}_\tau(\widetilde{\Bzeta}_{\tau0}(\Bx_0))-\widehat{Q}_\tau\left(\Bzeta^{\star}_\tau(\Bx_0)\right)$ in terms of a linear function of $\left\|\BJ_\tau^{1/2}\widetilde{\Bdelta}(\Bx_0)\right\|$, and a complementary lower bound in terms of a quadratic function. Finally, by combining these two bounds, we obtain the desired error bound.

\textbf{First proof that the deviation of the estimator $\widetilde{\Bdelta}(\Bx_0)$ lies in the set $A(e_0)$.}
 Define $\widehat{Q}_\tau(\Bzeta)=\sum_{i=1}^n\alpha_i(\Bx_0)\sum_{j=1}^{m_i}\frac{1}{m_i}\rho_\tau\left(Y_{ij}-\Bzeta^{\top}\BD_{ij}\right)$,$S_{ij}(\Bzeta)=\tau-I\left(Y_{ij}\leq \Bzeta^{\top}\BD_{ij}\right)$, 
 \begin{equation}
     \sum_{i=1}^n\alpha_i(\Bx_0)\sum_{j=1}^{m_i}\frac{1}{m_i}S_{ij}(\Bzeta)\BD_{ij}\in\nabla\widehat{Q}_\tau\big(\Bzeta\big).
 \end{equation}
By the convexity of $\widehat{Q}_\tau(\cdot)$, we have
	$$\widehat{Q}_\tau\big(\widetilde{\Bzeta}_{\tau0}(\Bx_0)\big)\geq \widehat{Q}_\tau\big(\Bzeta^{\star}_\tau(\Bx_0)\big)-\sum_{i=1}^n\alpha_i(\Bx_0)\sum_{j=1}^{m_i}\frac{1}{m_i}S_{ij}\left(\Bzeta^{\star}_\tau(\Bx_0)\right)\cdot \left\lbrace\widetilde{\Bzeta}_{\tau0}(\Bx_0)-\Bzeta^{\star}_\tau(\Bx_0)\right\rbrace^{\top}\BD_{ij}.$$
	
	\noindent By optimality of $\widetilde{\Bzeta}_\tau(\Bx_0)$ for the $\ell_1$-penalized problem, we have
	\begin{equation}
		\begin{aligned}
			0&\leq \widehat{Q}_\tau\left(\Bzeta^{\star}_\tau(\Bx_0)\right)-\widehat{Q}_\tau\left(\widetilde{\Bzeta}_{\tau0}(\Bx_0)\right)+\frac{\lambda_2}{n_{rf}}\left(\left\| \Bzeta^{\star}_\tau(\Bx_0)\right\| _1-\left\| \widetilde{\Bzeta}_{\tau0}(\Bx_0)\right\| _1\right)\\
			&\leq \sum_{i=1}^n \alpha_i(\Bx_0)\sum_{j=1}^{m_i}\frac{1}{m_i}S_{ij}\left(\Bzeta^{\star}_\tau(\Bx_0)\right)\BD_{ij}^{\top}\cdot\left\{\widetilde{\Bzeta}_{\tau0}(\Bx_0)-\Bzeta^{\star}_\tau(\Bx_0)\right\}\\
            &\quad+\frac{\lambda_2}{n_{rf}}\left(\left\| \Bzeta^{\star}_\tau(\Bx_0)\right\| _1-\left\| \widetilde{\Bzeta}_{\tau0}(\Bx_0)\right\| _1\right)\\
			&\leq \left\|\sum_{i=1}^n \alpha_i(\Bx_0)\sum_{j=1}^{m_i}\frac{1}{m_i}S_{ij}\left(\Bzeta^{\star}_\tau(\Bx_0)\right)\BD_{ij}\right\| _\infty\left\| \widetilde{\Bzeta}_{\tau0}(\Bx_0)-\Bzeta^{\star}_\tau(\Bx_0)\right\| _1\\
            &\quad+\frac{\lambda_2}{n_{rf}}\left(\left\| \Bzeta^{\star}_\tau(\Bx_0)\right\| _1-\left\| \widetilde{\Bzeta}_{\tau0}(\Bx_0)\right\| _1\right).\\
		\end{aligned}
		\nonumber
	\end{equation}
\noindent Then we bound $\left\|\sum_{i=1}^n \alpha_i(\Bx_0)\sum_{j=1}^{m_i}\frac{1}{m_i}S_{ij}\left(\Bzeta^{\star}_\tau(\Bx_0)\right)\BD_{ij}\right\| _\infty$. According to  a U-statistic concentration inequality and a union bound, with probability $1-\gamma$, we have
\begin{equation}
	\begin{aligned}
	&\quad\left\|\sum_{i=1}^n \alpha_i(\Bx_0)\sum_{j=1}^{m_i}S_{ij}\left(\Bzeta^{\star}_\tau(\Bx_0)\right)\BD_{ij}\right\| _\infty\\
    &\leq	\left\|\sum_{i=1}^n \alpha_i(\Bx_0)\mathbb{E}\left[ S_{ij}\left(\Bzeta^{\star}_\tau(\Bx_0)\right)\BD_{ij}\mid\BX_i\right] \right\| _\infty+\sqrt{\frac{s\log\left(\left(p_t+p_w \right)/\gamma  \right) }{n}}\\
		&\leq \left\|\sum_{i=1}^n\alpha_i(\Bx_0)\mathbb{E}\left[ \left\{S_{ij}\left(\Bzeta^{\star}_\tau(\Bx_0)\right)-S_{ij}\left(\Bzeta^{\star}_\tau(\BX_i)\right)\right\}\BD_{ij}\mid\BX_i\right] \right\| _\infty\\
        &\quad +\left\|\sum_{i=1}^n\alpha_i(\Bx_0)\mathbb{E}\left[ S_{ij}\left(\Bzeta^{\star}_\tau(\BX_i)\right)\BD_{ij}\mid\BX_i\right] \right\| _\infty+\sqrt{\frac{s\log\left(\left(p_t+p_w\right)/\gamma\right)}{n}}\\
        &=\left\|\sum_{i=1}^n\alpha_i(\Bx_0)\mathbb{E}\left[ \left\{F_{Y_{ij}\mid\BD_{ij}}\left(\Bzeta^{\star}_\tau(\Bx_0)^{\top}\BD_{ij}\right)-F_{Y_{ij}\mid\BD_{ij}}\left(\Bzeta^{\star}_\tau(\BX_i)^{\top}\BD_{ij}\right)\right\}\BD_{ij}\mid\BX_i\right] \right\| _\infty\\
        &\quad +\sqrt{\frac{s\log\left(\left(p_t+p_w \right)/\gamma\right)}{n}}\\
	&\leq \sqrt{k}\bar{f}Ls^{-\frac{1}{2\omega p_x}}+\sqrt{\frac{s\log\left(\left(p_t+p_w \right)/\gamma  \right) }{n}}\leq\frac{1}{c}\frac{\lambda_2}{n_{rf}}.
	\end{aligned}
\end{equation}
Then we have 
\begin{equation}
    0\leq\frac{1}{c}\frac{\lambda_2}{n_{rf}}\left\|\widetilde{\Bzeta}_{\tau0}(\Bx_0)-\Bzeta^{\star}_\tau(\Bx_0)\right\|_1+\frac{\lambda_2}{n_{rf}}\left\|\Bzeta^{\star}_\tau(\Bx_0)\right\| _1-\frac{\lambda_2}{n_{rf}}\left\| \widetilde{\Bzeta}_{\tau0}(\Bx_0)\right\| _1,
    \nonumber
\end{equation}
\begin{equation}
    -\frac{1}{c}\left\|\widetilde{\Bdelta}(\Bx_0)\right\|_1=-\frac{1}{c}||\widetilde{\Bzeta}_{\tau0}(\Bx_0)-\Bzeta^{\star}_\tau(\Bx_0)||_1\leq\left\|\Bzeta^{\star}_\tau(\Bx_0)\right\|_1-\left\|\widetilde{\Bzeta}_{\tau0}(\Bx_0)\right\|_1.
    \nonumber
\end{equation}
On the other hand, by applying the triangle inequality, we have
\begin{equation}
\begin{aligned}
&\quad\left\|\Bzeta^{\star}_\tau(\Bx_0)\right\|_1-\left\|\widetilde{\Bzeta}_{\tau0}(\Bx_0)\right\|_1\\
&=\left\|\Bzeta^{\star}_\tau(\Bx_0)_S\right\|_1+\left\|\Bzeta^{\star}_\tau(\Bx_0)_{S^C}\right\|_1-\left\|\widetilde{\Bzeta}_{\tau0}(\Bx_0)_S\right\|_1-\left\|\widetilde{\Bzeta}_{\tau0}(\Bx_0)_{S^C}\right\|_1\\
&\leq \left\|\Bzeta^{\star}_\tau(\Bx_0)_S-\widetilde{\Bzeta}_{\tau0}(\Bx_0)_S\right\|_1- \left\|\Bzeta^{\star}_\tau(\Bx_0)_{S^C}-\widetilde{\Bzeta}_{\tau0}(\Bx_0)_{S^C}\right\|_1\\
&=\left\|\widetilde{\Bdelta}(\Bx_0)_S\right\|_1-\left\|\widetilde{\Bdelta}(\Bx_0)_{S^C}\right\|_1.
\end{aligned}
\nonumber
\end{equation}
	Thus 
 $$\left\|\widetilde{\Bdelta}(\Bx_0)_S\right\|_1-\left\|\widetilde{\Bdelta}(\Bx_0)_{S^C}\right\|_1\geq -\frac{1}{c}\left\|\widetilde{\Bdelta}(\Bx_0)_S\right\|_1-\frac{1}{c}\left\|\widetilde{\Bdelta}(\Bx_0)_{S^C}\right\|_1,$$
which leads to $\left\|\widetilde{\Bdelta}(\Bx_0)_S\right\|_1\geq\frac{c-1}{c+1}\left\|\widetilde{\Bdelta}(\Bx_0)_{S^C}\right\|_1$ (i.e. $\widetilde{\Bdelta}(\Bx_0)\in A(\frac{c+1}{c_1}):= \{\Bdelta\in\mathbb{R}^{(p_t+p_w)}:\|\Bdelta_{S^c}\|_1\leq \frac{c+1}{c_1}\|\Bdelta_{S}\|_1\}$).
 
\textbf{Next, we get the upper bound of $\widehat{Q}_\tau(\widetilde{\Bzeta}_{\tau0}(\Bx_0))-\widehat{Q}_\tau\left(\Bzeta^{\star}_\tau(\Bx_0)\right)$.} We apply \eqref{lemma:restricted set.2} in the last inequality. Also by the optimality of $\widetilde{\Bzeta}_{\tau0}(\Bx_0)$, we have
\begin{equation}\label{eq22}
	\begin{aligned}
		&\widehat{Q}_\tau (\widetilde{\Bzeta}_{\tau0}(\Bx_0))-\widehat{Q}_\tau(\Bzeta^{\star}_\tau(\Bx_0))\leq\frac{\lambda_2}{n_{rf}}\|\Bzeta^{\star}_\tau(\Bx_0)\|_1-\frac{\lambda_2}{n_{rf}}\|\widetilde{\Bzeta}_{\tau0}(\Bx_0)\|_1\\
		\leq&\frac{\lambda_2}{n_{rf}}\|\widetilde{\Bdelta}(\Bx_0)_S\|_1
		\leq \frac{\lambda_2}{n_{rf}}\sqrt{k}\|\BJ_\tau^{1/2}\widetilde{\Bdelta}(\Bx_0)\|/\underline{f}^{1/2}t_0,
		\end{aligned}
\end{equation}
  where the last inequality follows from Equation (3.4) in Lemma 4 of \cite{belloni2011ℓ}. 
  
  \textbf{Then we derive the lower bound of $\widehat{Q}_\tau(\widetilde{\Bzeta}_{\tau0}(\Bx_0))-\widehat{Q}_\tau\left(\Bzeta^{\star}_\tau(\Bx_0)\right)$.} Using the Knight’s identity $\rho_\tau(x-y)-\rho_\tau(x) =-y(\tau- 1\{x\leq0\}) + \int_{0}^{y}\left( 1\{x\leq t\}-1\{x\leq0\}\right)dt$ and the U-statistic concentration inequality in \cite{hoeffding1963probability}, we have, with probability $1-\gamma$,
\begin{equation}\label{eq21}
\begin{aligned}
&\quad\widehat{Q}_\tau(\widetilde{\Bzeta}_{\tau0}(\Bx_0))-\widehat{Q}_\tau\left(\Bzeta^{\star}_\tau(\Bx_0)\right)\\   	&\geq\sum_{i=1}^{n}\alpha_i(\Bx_0)\mathbb{E}\left[\rho_{\tau }\left(Y_i-\widetilde{\Bzeta}_{\tau0}(\Bx_0)^{\top}\BD_i\right)-\rho_{\tau }\left(Y_{ij}-\Bzeta^{\star}_\tau(\Bx_0)^{\top}\BD_{ij}\right)\mid\BX_i\right]\\
        &\quad-\sqrt{\frac{s\log \left( 1/\gamma\right) }{n}}\\
   	&\geq\sum_{i=1}^{n}\alpha_i(\Bx_0)\mathbb{E}\left[\rho_{\tau }\left(Y_{ij}-\widetilde{\Bzeta}_{\tau0}(\Bx_0)^{\top}\BD_{ij}\right)-\rho_{\tau }\left(Y_{ij}-\Bzeta^{\star}_\tau(\Bx_0)^{\top}\BD_{ij}\right)\mid\Bx_0\right]\\
    &\quad-Ls^{-\frac{1}{2\omega p_x}}-\sqrt{\frac{s\log \left( 1/\gamma\right) }{n}}\\
   	&\geq \left(\|\BJ_\tau^{1/2}\widetilde{\Bdelta}(\Bx_0)\|^2/4\right)\wedge \left(t\|\BJ_\tau^{1/2}\widetilde{\Bdelta}(\Bx_0)\|\right)-Ls^{-\frac{1}{2\omega p_x}}-\sqrt{\frac{s\log \left( 1/\gamma\right) }{n}},
   	\end{aligned}
   \end{equation}
where the last inequality follows from~\eqref{lemma:restricted set.1} in Lemma~\ref{lemma:restricted set}. We let 
$$\mu:=\frac{2\lambda_2}{n_{rf}}\frac{\sqrt{k} }{\underline{f}^{1/2}t_0}+2\sqrt{\frac{\lambda_2^2}{n_{rf}^2}\frac{k }{\underline{f}t_0^2}+Ls^{-\frac{1}{2\omega p_x}}+\left(\frac{s\log\left( 1/\gamma\right)}{n}\right)^{1/2}}.$$

\textbf{Finally, we employ the method of proof by contradiction to derive an upper bound for the error.} If $\|\BJ_\tau\widetilde{\Bdelta}(\Bx_0)\|>\mu$, with the growth condition \eqref{eq18}, we have $t\|\BJ_\tau^{1/2}\widetilde{\Bdelta}(\Bx_0)\|\geq\|\BJ_\tau^{1/2}\widetilde{\Bdelta}(\Bx_0)\|^2/4$. Combine \eqref{eq21} and \eqref{eq22},
$$0>\frac{\lambda_2}{n_{rf}}\sqrt{k}\|\BJ_\tau^{1/2}\widetilde{\Bdelta}(\Bx_0)\|/\underline{f}^{1/2}t_0-\|\BJ_\tau^{1/2}\widetilde{\Bdelta}(\Bx_0)\|^2/4+Ls^{-\frac{1}{2\omega p_x}}+\sqrt{\frac{s\log \left( 1/\gamma\right) }{n}}\geq 0,$$
which leads to contradiction. Hence, it must hold that $\|\BJ_\tau^{1/2}\widetilde{\Bdelta}(\Bx_0)\|\leq \mu$. Combining this result with inequality~\eqref{lemma:restricted set.2} in Lemma~\ref{lemma:restricted set}, Theorem~\ref{thm:beta_nonsmooth} is proved.
\end{proof}

\subsection{Proof of Results in Section 3.2}
To obtain theoretical results for $\widehat{\Btheta}(\Bx_0)$, we first introduce some notations. Recall that the orthogonal score function, as defined in Equation (3) of the main text, is 
\begin{equation}\label{orthogonal}
\Bpsi_\tau(\BZ_{ij};\Btheta,\Bmeta)
= \varphi_\tau\bigl(Y_{ij} - \Btheta(\BX_i)^\top \BT_{ij} - \Bbeta(\BX_i)^\top \BW_{ij}\bigr)\;\bigl\{\BT_{ij} - \BL(\BX_{i})^\top \BW_{ij}\bigr\}.
\end{equation}
We let
$$m(\Bx;\Btheta,\Bmeta)=\mathbb{E}\big[\Bpsi_\tau(\BZ_{ij};\Btheta,\Bmeta)\mid \BX=\Bx\big]$$
denote the expected score function, 
$$\Psi_0(\Bx_0;\Btheta,\Bmeta)=\sum_{i=1}^{n}\alpha_i(\Bx_0)m (\BX_i;\Btheta,\Bmeta)$$
denote the weighted expected score function and
$$\Psi(\Bx_0;\Btheta,\Bmeta)=\sum_{i=1}^{n}\alpha_i(\Bx_0)\sum_{j=1}^{m_i}\frac{1}{m_i}\Bpsi_\tau(\BZ_{ij};\Btheta,\Bmeta)$$
denote the weighted empirical score function.

	\begin{lemma}\label{lemma1}
 Under Assumptions~\ref{A3.5}-\ref{A3.6},
 \begin{equation}\label{eq:lemmaS.3}
     \sup_{\Btheta\in\Theta,\|\Bmeta-\Bmeta^{\star}(\Bx_0)\|\leq \chi_n}||m(\Bx_0;\Btheta,\Bmeta)-\Psi(\Bx_0;\Btheta,\Bmeta)||=o_p(1).
 \end{equation}
	\end{lemma}
	
	\begin{proof}
		We decompose \eqref{eq:lemmaS.3} into
		\begin{equation}
			\begin{aligned}
				&\quad\sup_{\Btheta\in\Theta,\|\Bmeta-\Bmeta^{\star}(\Bx_0)\|\leq \chi_n}\left\|m(\Bx_0;\Btheta,\Bmeta)-\Psi(\Bx_0;\Btheta,\Bmeta)\right\|\\
                &\leq \sup_{\Btheta\in\Theta,\|\Bmeta-\Bmeta^{\star}(\Bx_0)\|\leq \chi_n}\left\|m(\Bx_0;\Btheta,\Bmeta)-\Psi_0(\Bx_0;\Btheta,\Bmeta)\right\|\\
                &\quad+\sup_{\Btheta\in\Theta,\|\Bmeta-\Bmeta^{\star}(\Bx_0)\|\leq \chi_n}\left\|\Psi_0(\Bx_0;\Btheta,\Bmeta)-\Psi(\Bx_0;\Btheta,\Bmeta)\right\|.
			\end{aligned}
		\end{equation}
		
\textbf{First, we bound the term $\sup_{\Btheta\in\Theta,\|\Bmeta-\Bmeta^{\star}(\Bx_0)\|\leq \chi_n}\left\|m(\Bx_0;\Btheta,\Bmeta)-\Psi_0(\Bx_0;\Btheta,\Bmeta)\right\|$.} By Proposition~\ref{thm:shrinkage}, we have
		 $\sup_{\Btheta,\|\Bmeta-\Bmeta^{\star}(\Bx_0)\|\leq \chi_n}||m(\Bx_0;\Btheta,\Bmeta)-\Psi_0(\Bx_0;\Btheta,\Bmeta)||= O(s^{-1/(2\omega p_x)}).$
		
\textbf{Next we turn to the term $\sup_{\Btheta,\|\Bmeta-\Bmeta^{\star}(\Bx_0)\|\leq \chi_n}||\Psi_0(\Bx_0;\Btheta,\Bmeta)-\Psi(\Bx_0;\Btheta,\Bmeta)||$.} We need to show that for any $\epsilon>0$,
		\begin{equation}\label{A}
			\mathbb{P}\left( \sup_{\Btheta,\|\Bmeta-\Bmeta^{\star}(\Bx_0)\|\leq \chi_n}\left\| \Psi_0(\Bx_0;\Btheta,\Bmeta)-\Psi(\Bx_0;\Btheta,\Bmeta)\right\| >\epsilon\right)=o(1).
		\end{equation}
Denote the parameter space $\Btheta\in\Theta$, where $\Theta$ is a compact subset of $\mathbb{R}^{p_t}$.  Partition $\Theta$ uniformly into $L_n:=\lceil\frac{n}{s}\rceil$ disjoint cubes $\Gamma_l$ with diameters less than $d_n=p_t\left( \frac{s}{n}\right)^{1/p_t} $. Let $\Bxi_l$ be the center of the $l$-th cube $\Gamma_l$. Note that 
		\begin{equation}
			\begin{aligned}\label{ED}
				&\sup_{\Btheta\in\Theta,\|\Bmeta-\Bmeta^{\star}(\Bx_0)\|\leq \chi_n}\left\| \Psi_0(\Bx_0;\Btheta,\Bmeta)-\Psi(\Bx_0;\Btheta,\Bmeta)\right\| \\				&\leq \max_l\sup_{\Btheta\in\Gamma_l,\left\| \Bmeta-\Bmeta^{\star}(\Bx_0)\right\|\leq\chi_n }\left\| \Psi_0(\Bx_0;\Btheta,\Bmeta)-\Psi_0(\Bx_0;\Bxi_l,\Bmeta)\right\|\\
                &\quad+\max_l\sup_{\Btheta\in\Gamma_l,\left\| \Bmeta-\Bmeta^{\star}(\Bx_0)\right\|\leq\chi_n }\left\| \Psi(\Bx_0;\Btheta,\Bmeta)-\Psi(\Bx_0;\Bxi_l,\Bmeta)\right\|\\
                &\quad+\max_l\sup_{\left\| \Bmeta-\Bmeta^{\star}(\Bx_0)\right\|\leq\chi_n }\left\| \Psi(\Bx_0;\Bxi_l,\Bmeta)-\Psi_0(\Bx_0;\Bxi_l,\Bmeta)\right\|.
			\end{aligned}
		\end{equation}

We first consider the first term of the right side of \eqref{ED}. 
It is easy to derive that
		\begin{equation}\label{E}
			\begin{aligned}
				&\quad\left\| \Bpsi_\tau(\BZ_{ij};\Btheta,\Bmeta)-\Bpsi_\tau(\BZ_{ij};\Bxi_l,\Bmeta)\right\| \\
                &=\left\|  I\left(Y_{ij}\leq \Btheta^{\top}\BT_{ij}+\Bbeta^{\top}\BW_{ij}\right)-I\left(Y_{ij}\leq \Bxi_l^{\top}\BT_{ij}+\Bbeta^{\top}\BW_{ij}\right) \left( \BT_{ij}-\BL^{\top}\BW_{ij}\right)\right\|  \\
				&\leq \left\|\left\lbrace I\left(\left|Y_{ij}- \Bxi_l^{\top}\BT_{ij}-\Bbeta^{\top}\BW_{ij}\right|\leq \left| (\Bxi_l-\Btheta)^{\top}\BT_{ij}\right|\right)\right\rbrace\left(\BT_{ij}-\BL^{\top}\BW_{ij}\right)\right\|\\
				&\leq \left\|\left\lbrace I\left(  | Y_{ij}- \Bxi_l^{\top}\BT_{ij}-\Bbeta^{\top}\BW_{ij}|\leq d_n\left\| \BT_{ij}\right\|\right)  \right\rbrace(\BT_{ij}-\BL^{\top}\BW_{ij})\right\|.
			\end{aligned}
		\end{equation}
Thus, the first term of the right side of \eqref{ED} satisfies
		\begin{equation}
			\begin{aligned}\label{eq39}
				&\quad\max_l\sup_{\Btheta\in\Gamma_l,\left\| \Bmeta-\Bmeta^{\star}(\Bx_0)\right\| \leq\chi_n}\left\| m(\Bx_0;\Btheta,\Bmeta)-m(\Bx_0;\Bxi_l,\Bmeta)\right\| \\
				&\leq\max_l\sup_{\Btheta\in\Gamma_l,\left\| \Bmeta-\Bmeta^{\star}(\Bx_0)\right\| \leq\chi_n}\bigg\| \mathbb{E}\bigg[ I\left(| Y_{ij}- \Bxi_l^{\top}\BT_{ij}-\Bbeta^{\top}\BW_{ij}|\leq d_n\left\| \BT_{ij}\right\|\right)\\
                &\quad\cdot\left(\BT_{ij}-\BL^{\top}\BW_{ij}\right)\mid \Bx_0\bigg]\bigg\| \\
			&=\max_l\sup_{\Btheta\in\Gamma_l,\left\| \Bmeta-\Bmeta^{\star}(\Bx_0)\right\| \leq\chi_n}\bigg\| \mathbb{E}\bigg[\int_{\Bxi_l^{\top}\BT_{ij}+\Bbeta^{\top}\BW_{ij}- d_n\left\|\BT_{ij}\right\|}^{\Bxi_l^{\top}\BT_i+\Bbeta^{\top}\BW_i+d_n\left\| \BT_{ij}\right\|}f(u|\BT_{ij},\BW_{ij})du\\
                &\quad\cdot(\BT_{ij}-\BL^{\top}\BW_{ij})du \mid \Bx_0\bigg]\bigg\| \\
			&\leq \max_l\sup_{\Btheta\in\Gamma_l,\left\| \Bmeta-\Bmeta^{\star}(\Bx_0)\right\| \leq\chi_n}2\bar{f}d_n\cdot\left\| \mathbb{E}\left[\left\| \BT_{ij}\right\| (\BT_{ij}-\BL^{\top}\BW_{ij})\mid \Bx_0 \right]\right\| .
			\end{aligned}
		\end{equation}
Note that $d_n\rightarrow0$ and $\left\| \mathbb{E}\left[\left\| \BT_{ij}\right\| (\BT_{ij}-\BL^{\top}\BW_{ij}) \mid \Bx_0\right]\right\| <\infty$, then the left side of equation \eqref{eq39} converges to 0. 

Therefore, the left side of equation \eqref{A} can be bounded by the sum of the following two terms:		
		\begin{equation}\label{C}			P_1=\mathbb{P}\left(\max_l\sup_{\Btheta\in\Gamma_l,\left\|\Bmeta-\Bmeta^{\star}(\Bx_0)\right\|\leq\chi_n }\left\| \Psi(\Bx_0;\Btheta,\Bmeta)-\Psi(\Bx_0;\Bxi_l,\Bmeta)\right\| >\frac{\epsilon}{2}\right) 
		\end{equation}
		and
		\begin{equation}\label{D}
			P_2=\mathbb{P}\left( \max_l\sup_{\left\| \Bmeta-\Bmeta^{\star}(\Bx_0)\right\|\leq\chi_n }\left\| \Psi(\Bx_0;\Bxi_l,\Bmeta)-\Psi_0(\Bx_0;\Bxi_l,\Bmeta)\right\| >\frac{\epsilon}{2}\right). 
		\end{equation}
        
		For $P_1$, define the random variable
        $$G_i=\left\| \sum_{j=1}^{m_i}\frac{1}{m_i}I\left(  \left| Y_{ij}- \Bxi_l^{\top}\BT_{ij}-\Bbeta^{\top}\BW_{ij}\right|\leq d_n\left\| \BT_{ij}\right\|  \right)\cdot\left( \BT_{ij}-\BL^{\top}\BW_{ij}\right)\right\| $$
        and its sub-Gaussian norm as $C_4=\|A_i\|_{\psi_2}$.Since $A_i$ is sub-Gaussian, according to  the Hoeffding inequality of the sub-Gaussian variable, then
		\begin{equation}
			\begin{aligned}
				\mathbb{P}\left(\left|\sum_{i=1}^{n} \alpha_i(G_i-\mathbb{E}G_i)\right|>\frac{\epsilon}{2}\right) \leq\exp\left(-\frac{\epsilon^2}{4C_4^2\alpha^*} \right)\rightarrow0,
			\end{aligned}
		\end{equation}
		where $\alpha^*=\sum_{i=1}^{n}\alpha_i^2=O_p\left(\frac{s}{n}\right)$. Combine with the inequality in \eqref{E} and the fact that $$\max_l\sup_{\Btheta\in\Gamma_l,\left\| \Bmeta-\Bmeta^{\star}(x_0)\right\| \leq\chi_n}\left\| m(\BX_i;\Btheta,\Bmeta)-m(\BX_i;\Bxi_l,\Bmeta)\right\|=o(1),$$ therefore we have $P_1=o(1).$
		
		For $P_2$, we define the random variable
        $$B_i=\left\| \sum_{j=1}^{m_i}\frac{1}{m_i}\left\lbrace I\left( Y_{ij}\leq \Bxi_l^{\top}\BT_{ij}+\Bbeta^{\top}\BW_{ij}\right)-\tau\right\rbrace\cdot\left( \BT_{ij}-\BL^{\top}\BW_{ij}\right)\right\|, $$
        and $C_5=\|B_i\|_{\psi_2}$, again apply the Hoeffding inequality for sub-Gaussian variable, 
		\begin{equation}
			\begin{aligned}
				&\mathbb{P}\left( \max_l\sup_{\left\| \Bmeta-\Bmeta^{\star}(\Bx_0)\right\|\leq\chi_n }\left\| \sum_{i=1}^{n}\alpha_i\left(\sum_{j=1}^{m_i}\frac{1}{m_i}\Bpsi_\tau(\BZ_{ij};\Bxi_l,\Bmeta)-\mathbb{E}\left[\Bpsi_\tau(\BZ_{ij};\Bxi_l,\Bmeta) \mid \BX_i\right]  \right) \right\| >\frac{\epsilon}{2}\right) \\
				&\leq\exp\left(-\frac{\epsilon^2}{4C_5^2\alpha^*} \right)\rightarrow0.
			\end{aligned}
			\nonumber
		\end{equation} 
	\end{proof}

\noindent \textbf{Proof of Theorem 1:} 	
\begin{proof}
 According to triangular inequality, we have
 \begin{equation}
     \begin{aligned}
         \left\| m(\Bx_0;\widehat{\Btheta}(\Bx_0),\widetilde{\Bmeta}(\Bx_0))\right\| \leq&\left\| m(\Bx_0;\widehat{\Btheta}(\Bx_0),\widetilde{\Bmeta}(\Bx_0))-\Psi(\Bx_0;\widehat{\Btheta}(\Bx_0),\widetilde{\Bmeta}(\Bx_0))\right\|\\
         &+\left\| \Psi(\Bx_0;\widehat{\Btheta}(\Bx_0),\widetilde{\Bmeta}(\Bx_0))\right\|.
     \end{aligned}
     \nonumber
 \end{equation}
According to Lemma \ref{lemma1},  $\left\| m(\Bx_0;\widehat{\Btheta}(\Bx_0),\widetilde{\Bmeta}(\Bx_0))-\Psi(\Bx_0;\widehat{\Btheta}(\Bx_0),\widetilde{\Bmeta}(\Bx_0))\right\| =o_p(1).$ According to Assumption~\ref{A3.7}, $\left\| \Psi(\Bx;\widehat{\Btheta}(\Bx_0),\widetilde{\Bmeta}(\Bx_0))\right\| =O_p\left(\max\{\alpha_i\}\right)=o_p(1)$. Together with Lemma~\ref{lemma1}, $\left\| m(\Bx_0;\widehat{\Btheta}(\Bx_0),\widetilde{\Bmeta}(\Bx_0))\right\|=o_p(1)$. Since $m(\Bx_0;\widehat{\Btheta}(\Bx_0),\Bmeta)$ is $L-$Lipschitz in $\Bmeta$,
\begin{equation}
    \begin{aligned}
        &\quad\mathbb{E}\left[ \left\| m(\Bx_0;\widehat{\Btheta}(\Bx_0),\Bmeta^{\star}(\Bx_0))-m(\Bx_0;\widehat{\Btheta}(\Bx_0),\widetilde{\Bmeta}(\Bx_0))\right\| \right]\\
        &\leq L\mathbb{E}\left[ \left\| \Bmeta^{\star}(\Bx_0)-\widetilde{\Bmeta}(\Bx_0)\right\| \mid \Bx_0\right] =o(1),
    \end{aligned}
    \nonumber
\end{equation}
which implies $\left\| m(\Bx_0;\widehat{\Btheta}(\Bx_0),\Bmeta^{\star}(x_0))\right\| =o_p(1).$
		
		Since $\Btheta=\Btheta^{\star}(\Bx_0)$ is the unique solution of the moment condition $m(\Bx_0;\Btheta,\Bmeta^{\star}(\Bx_0))=0$ , for any $\upsilon>0$, there exists a positive $\varsigma$, such that $\mathbb{P}\left[ \left\| \widehat{\Btheta}(\Bx_0)-\Btheta^{\star}(\Bx_0)\right\| \geq\upsilon\right] \leq\mathbb{P}\left[ \left\| m(\Bx;\widehat{\Btheta}(\Bx_0),\Bmeta^{\star}(\Bx_0))\right\| \geq\varsigma\right] $. The probability on the right hand side converges to 0, thus $\left\| \widehat{\Btheta}(\Bx_0)-\Btheta^{\star}(\Bx_0)\right\| =o_p(1)$.
\end{proof}

\textbf{Next we prove the convergence rate of $\widehat{\Btheta}(\Bx_0)$.} Before that, we establish a lemma to bound $\left\|m(\Bx_0;\Btheta,\widetilde{\Bmeta}(\Bx_0))-\Psi(\Bx_0;\Btheta,\widetilde{\Bmeta}(\Bx_0))\right\|$.

\begin{lemma}\label{S5}
Under Assumptions~\ref{A3.5}~\ref{A3.6}, for any $\Btheta\in\Theta$ and for any $\Bmeta$ that satisfies $\|\Bmeta-\Bmeta^*(\Bx)\|\leq \chi_n\rightarrow 0$, with probability $1-\gamma$, 
\begin{equation}
	\sup_{\Btheta\in\Theta,\|\Bmeta-\Bmeta^*(\Bx_0)\|\leq \chi_n}\left\|m(\Bx_0;\Btheta,\Bmeta)-\Psi(\Bx_0;\Btheta,\Bmeta)\right\|=O\left(s^{-\frac{1}{2\omega p_x}}+\sqrt{\frac{s\log\left(1/\gamma\right)}{n}}\right).
\end{equation}
Furthermore, 
\begin{equation}\label{22}
	\sup_{\Btheta\in\Theta,\|\Bmeta-\Bmeta^*(\Bx_0)\|\leq \chi_n}\mathbb{E}\left[ \left\| m(\Bx_0;\Btheta,\Bmeta)-\Psi(\Bx_0;\Btheta,\Bmeta)\right\| \right] =O\left(s^{-\frac{1}{2\omega p_x}}+\sqrt{\frac{s}{n}}\right).
\end{equation}
Here, $\omega$ is defined as in Assumption~\ref{sparsity level}
\end{lemma}
\begin{proof}
    The proof of Lemma~\ref{S5} follows directly by applying Hoeffding's inequality for U-statistics and Proposition~\ref{thm:shrinkage}.
\end{proof}

\noindent \textbf{Proof of Theorem 2:} 
\begin{proof}
We first recall the notation: $k$ is defined in Assumption~\ref{assum:coeff} and $\omega$ is defined in Assumption~\ref{sparsity level}.

By Taylor expansion, we have
$$m(\Bx_0;\widehat{\Btheta}(\Bx_0),\widetilde{\Bmeta}(\Bx_0))=m(\Bx_0;\Btheta^{\star}(\Bx_0),\Bmeta^{\star}(\Bx_0))+\bm{M}(\Bx_0)\left\{\widehat{\Btheta}(\Bx_0)-\Btheta^{\star}(\Bx_0) \right\}+\bm{\varrho},$$
where $\bm{\varrho}$ is a random variable such that $\left\|\bm{\varrho}\right\|=O\left(\|\widetilde{\Bmeta}(\Bx_0)-\Bmeta^{\star}(\Bx_0)\| ^2+\| \widehat{\Btheta}(\Bx_0)-\Btheta^{\star}(\Bx_0)\|^2 \right)$ and $\bm{M}(\Bx_0)=\frac{\partial}{\partial\Btheta}m(\Bx_0;\Btheta,\Bmeta^{\star}(\Bx_0))|_{\Btheta=\Btheta^{\star}(\Bx_0)}$. Then
		$$\widehat{\Btheta}(\Bx_0)-\Btheta^{\star}(\Bx_0)=\bm{M}(\Bx_0)^{-1}\left( m(\Bx_0;\widehat{\Btheta}(\Bx_0),\widetilde{\Bmeta}(\Bx_0))-\bm{\varrho}\right),$$
        $$\mathbb{E}\left[ \left\|\widehat{\Btheta}(\Bx_0)-\Btheta^{\star}(\Bx_0) \right\|\right]=O\left(\mathbb{E}\left[\left\|m(\Bx_0;\widehat{\Btheta}(\Bx_0),\widetilde{\Bmeta}(\Bx_0))-\bm{\varrho}\right\|\right]\right).$$
        By the triangular inequality, 
        \begin{equation}
            \begin{aligned}
               &\quad\mathbb{E}\left[\left\|m(\Bx_0;\widehat{\Btheta}(\Bx_0),\widetilde{\Bmeta}(\Bx_0))-\bm{\varrho}\right\|\right]\\
               &\leq  \mathbb{E}\left[\left\|m(\Bx_0;\widehat{\Btheta}(\Bx_0),\widetilde{\Bmeta}(\Bx_0))-\Psi(\Bx_0;\widehat{\Btheta}(\Bx_0),\widetilde{\Bmeta}(\Bx_0))\right\|\right]+ \mathbb{E}\left[\left\|\Psi(\Bx_0;\widehat{\Btheta}(\Bx_0),\widetilde{\Bmeta}(\Bx_0))\right\|\right]\\
               &\quad+\mathbb{E}\left[\left\| \widetilde{\Bmeta}(\Bx_0)-\Bmeta^{\star}(\Bx_0)\right\|^2 \right] +\mathbb{E}\left[ \left\|\widehat{\Btheta}(\Bx_0)-\Btheta^{\star}(\Bx_0) \right\|^2\right]. 
            \end{aligned}
            \nonumber
        \end{equation}
		The first term can be bounded by $\mathbb{E}\left[ \left\|m(\Bx_0;\widehat{\Btheta}(\Bx_0),\widetilde{\Bmeta}(\Bx_0))-\Psi(\Bx_0;\widehat{\Btheta}(\Bx_0),\widetilde{\Bmeta}(\Bx_0))\right\|\right]=O\left( s^{-\frac{1}{2\omega p_x}}+\sqrt{\frac{s}{n}}\right)$ according to \eqref{22}. By Assumption~\ref{A3.7}, $\mathbb{E}\left[\left\|\Psi(\Bx_0;\widehat{\Btheta}(\Bx_0),\widetilde{\Bmeta}(\Bx_0))\right\|\right]\leq C\max \{\alpha_i\}=O_p\left( \frac{s}{n}\right) .$
		By Proposition~\ref{thm:nuisance_error} and Theorem~\ref{thm_conv}, the nuisance estimator satisfies $\mathbb{E}\left[\left\| \widetilde{\Bmeta}(\Bx_0)-\Bmeta^{\star}(\Bx_0)\right\|^2\right]=O\left(k^2\cdot s^{-\frac{1}{\omega p_x}}+\frac{k^2s\log(p_t+p_w)}{n} \right).$ Finally, by the consistency of $\widehat{\Btheta}(\Bx_0)$, the last term $\mathbb{E}\left[ \left\|\widehat{\Btheta}(\Bx_0)-\Btheta^{\star}(\Bx_0) \right\|^2\right]$ can be ignored. Thus we have 
		$$\mathbb{E}\left[ \left\|\widehat{\Btheta}(\Bx_0)-\Btheta^{\star}(\Bx_0) \right\|\right]=O\left( s^{-\frac{1}{2\omega p_x}}+\sqrt{\frac{s}{n}}\right).$$
\end{proof}

\noindent \textbf{Proof of Theorem 3:} 
\begin{proof}
In the following proof, we recall that $k$ is defined in Assumption~\ref{assum:coeff}, $\omega$ in Assumption~\ref{sparsity level} and $\sigma_n(\Bx_0,\bm{a})$ in Theorem 3 in the main text.

We begin by defining an intermediate variable $\bar{\Btheta}(\Bx_0)=\Btheta^{\star}(\Bx_0)+\sum_{i=1}^{n}\alpha_i(\Bx_0)\bm{\rho}_i^*$, where $\bm{\rho}_i^*=-\bm{M}(\Bx_0)^{-1}\sum_{j=1}^{m_i}\frac{1}{m_i}\Bpsi_\tau\left(\BZ_{ij};\Btheta^{\star}(\Bx_0),\Bmeta^{\star}(\Bx_0)\right)$. Such variable can be regarded as a tractable oracle-type quantity, which can be shown to be asymptotically normal but is infeasible in practice. We then demonstrate that the deviation between $\bar{\Btheta}(\Bx_0)$ and the proposed estimator $\widetilde{\Btheta}(\Bx_0)$ is asymptotically negligible.
    
\textbf{Consider the intermediate variable $\bar{\Btheta}(\Bx_0)$.} According to Theorem 1 in \citep{wager2018estimation}, $\sigma_n(\Bx_0,\bm{a})^{-1}\left\langle \bm{a},\bar{\Btheta}(\Bx_0)-\Btheta^{\star}(\Bx_0)\right\rangle\rightarrow_d\mathcal{N}(0,1).$ 

\textbf{Then it suffices to show that $\sigma_n(\Bx_0,\bm{a})^{-1}\left\langle \bm{a},\Btheta^{\star}(\Bx_0)-\bar{\Btheta}(\Bx_0)\right\rangle=o_p(1)$.}  By Taylor's expansion, we have
\begin{equation}
	\begin{aligned}
		&\quad\sigma_n(\Bx_0,\bm{a})^{-1}\left\langle \bm{a},\widehat{\Btheta}(\Bx_0)-\bar{\Btheta}(\Bx_0)\right\rangle\\
        &=	\sigma_n(\Bx_0,\bm{a})^{-1}\left\langle \bm{a},\bm{M}(\Bx_0)^{-1}\left\{m(\Bx_0;\widehat{\Btheta}(\Bx_0),\widetilde{\Bmeta}(\Bx_0))+\Psi(\Bx_0;\Btheta^{\star}(\Bx_0),\Bmeta^{\star}(\Bx_0)) +\left\|\bm{\varrho}\right\|\right\}\right\rangle.
	\end{aligned}
\nonumber
\end{equation}
Recall that $\left\|\bm{\varrho}\right\|=O\left(\|\widetilde{\Bmeta}(\Bx_0)-\Bmeta^{\star}(\Bx_0)\| ^2+\| \widehat{\Btheta}(\Bx_0)-\Btheta^{\star}(\Bx_0)\|^2 \right)$. This term is of higher order and therefore negligible relative to the remainder term. Then we only need to show that
\begin{equation}\label{an proof}
    \sigma_n^{-1}(\Bx_0,\bm{a})\left\| m(\Bx_0;\widehat{\Btheta}(\Bx_0),\widetilde{\Bmeta}(\Bx_0))+\Psi(\Bx_0;\Btheta^{\star}(\Bx_0),\Bmeta^{\star}(\Bx_0))\right\|=o_p(1).
\end{equation}
The left side of \eqref{an proof} can be decomposed as
\begin{equation}\label{error_decomposition}
	\begin{aligned}
	&\quad\left\|\Psi(\Bx_0;\Btheta^{\star}(\Bx_0),\Bmeta^{\star}(\Bx_0))+m(\Bx_0;\widehat{\Btheta}(\Bx_0),\widetilde{\Bmeta}(\Bx_0))\right\|\\
    &\leq\left\|\Psi_0(\Bx_0;\widehat{\Btheta}(\Bx_0),\Bmeta^{\star}(\Bx_0))+\Psi(\Bx_0;\Btheta^{\star}(\Bx_0),\Bmeta^{\star}(\Bx_0)) \right\|\\
    &~~~~~~~~~~~~~~~~~~~~~~~~~~~~~+\left\| m(\Bx_0;\widehat{\Btheta}(\Bx_0),\widetilde{\Bmeta}(\Bx_0))-\Psi_0(\Bx;\widehat{\Btheta}(\Bx),\Bmeta^{\star}(\Bx_0))\right\|  \\
    &\leq\left\| \Psi_0(\Bx_0;\widehat{\Btheta}(\Bx_0),\Bmeta^{\star}(\Bx_0))-\Psi(\Bx_0;\widehat{\Btheta}(\Bx_0),\Bmeta^{\star}(\Bx_0))\right.\\
    &~~~~~~~~~~~~~~~~~~~~~~~~~~\left.-\left\lbrace\Psi_0(\Bx_0;\Btheta^{\star}(\Bx_0),\Bmeta^{\star}(\Bx_0))-\Psi(\Bx_0;\Btheta^{\star}(\Bx_0),\Bmeta^{\star}(\Bx_0)) \right\rbrace\right\|\\
    &\quad+\left\|\Psi(\Bx_0;\widehat{\Btheta}(\Bx_0),\Bmeta^{\star}(\Bx_0))\right\| +\left\|\Psi_0(\Bx;\Btheta^{\star}(\Bx_0),\Bmeta^{\star}(\Bx_0)) \right\|\\
    &\quad+\left\| m(\Bx_0;\widehat{\Btheta}(\Bx_0),\Bmeta^{\star}(\Bx_0))-\Psi_0(\Bx_0;\widehat{\Btheta}(\Bx_0),\Bmeta^{\star}(\Bx_0))\right\|\\
    &\quad+\left\| m(\Bx_0;\widehat{\Btheta}(\Bx_0),\widetilde{\Bmeta}(\Bx_0))-m(\Bx_0;\widehat{\Btheta}(\Bx_0),\Bmeta^{\star}(\Bx_0))\right\|.
	\end{aligned}
\end{equation}
To proceed, we control the five terms in the left side of~\eqref{error_decomposition} respectively. Begin with the first term 
\begin{equation}
    \begin{aligned}
        &\quad\left\| \delta\left((\Btheta^{\star}(\Bx_0),\Bmeta^{\star}(\Bx_0)),(\widehat{\Btheta}(\Bx_0),\Bmeta^{\star}(\Bx_0))\right) \right\|\\
        &:=\Big\| \Psi_0(\Bx_0;\widehat{\Btheta}(\Bx_0),\Bmeta^{\star}(\Bx_0))-\Psi(\Bx_0;\widehat{\Btheta}(\Bx_0),\Bmeta^{\star}(\Bx_0))\\
        &~~~~~~~~~~~~~~~~~~~~~~~~~~~~~~~~~-\left\lbrace\Psi_0(\Bx_0;\Btheta^{\star}(\Bx_0),\Bmeta^{\star}(\Bx_0))-\Psi(\Bx_0;\Btheta^{\star}(\Bx_0),\Bmeta^{\star}(\Bx_0)) \right\rbrace\Big\|.
    \end{aligned}
    \nonumber
\end{equation}
Apply the conclusion in Equation \eqref{eq39} again, for any $\Btheta_1,\Btheta_2\in\Theta$, we have
\begin{equation}
	\begin{aligned}
&\quad\mathbb{E}\left[\left\|\sum_{i=1}^{n}\alpha_i(\Bx_0)\left\lbrace\sum_{j=1}^{m_i}\frac{1}{m_i}\psi(\BZ_{ij};\Btheta_1,\Bmeta^{\star}(\Bx_0))-\sum_{j=1}^{m_i}\frac{1}{m_i}\psi\left(\BZ_{ij};\Btheta_2,\Bmeta^{\star}(\Bx_0)\right)\right\rbrace \right\|^2\mid\Bx_0\right]\\
&=\mathbb{E}\bigg[\bigg\|\sum_{i=1}^{n}\alpha_i(\Bx_0)\sum_{j=1}^{m_i}\frac{1}{m_i}\left\lbrace I\left( Y_{ij}-\Bbeta^{\star}(\Bx_0)^{\top}\BW_{ij}-\Btheta_2^{\top}\BT_i\leq0 \right)\right.\\
&~~~~~~~~~~~~~~~~~~~\left.-I\left( Y_{ij}-\Bbeta^{\star}(\Bx_0)^{\top}\BW_{ij}-\Btheta_1^{\top}\BT_{ij}\leq0\right)  \right\rbrace\cdot\left\lbrace\BT_{ij}-\BL^{\star}(\Bx_0)^{\top}\BW_{ij} \right\rbrace \bigg\|^2\mid\Bx_0\bigg]\\	&\leq\mathbb{E}\bigg[\bigg\|\sum_{i=1}^{n}\alpha_i(\Bx_0)\sum_{j=1}^{m_i}I\left( \left| Y_{ij}-\Bbeta^{\star}(\Bx_0)^{\top}\BW_{ij}-\Btheta_1^{\top}\BT_{ij}\right| \leq\left|(\Btheta_1-\Btheta_2)^{\top}\BT_{ij} \right| \right)\\
&\quad\cdot\left\lbrace\BT_{ij}-\BL^{\star}(\Bx_0)^{\top}\BW_{ij} \right\rbrace \bigg\|^2\mid\Bx_0\bigg]\\
&\leq p_t\sigma_e^2\bar f\|\Btheta_1-\Btheta_2\|,
	\end{aligned}
\nonumber
\end{equation}
where $\bar f$ is defined in Assumption~\ref{assum:density} and $\sigma_e^2=\max_{\nu=1,\dots,p_t}var(e_{ij}^{(\nu)}).$
Hence, if $\|\Btheta_1-\Btheta_2\|\leq\varpi<1$, we have $\|\Psi\left(\Bx;\Btheta_1,\Bmeta^{\star}(\Bx_0)\right)-\Psi\left(\Bx;\Btheta_2,\Bmeta^{\star}(\Bx_0)\right)\|\leq\sqrt{p_t\sigma_e^2\bar f\varpi}$. We can uniformly partition the parameter
space $\Theta$ into $\lceil\left\lbrace\sqrt{p_t}\varpi/(p_t\sigma_e^2)\bar f\right\rbrace^{p_t}\rceil$ disjoint small cubes $\Gamma_l$, $l=1,\dots,\left\lceil\left\lbrace\sqrt{p_t}\varpi/(p_t\sigma_e^2\bar f)\right\rbrace^{p_t}\right\rceil$. For any $\Btheta_1,\Btheta_2\in\Gamma_l$, $\|\Btheta_1-\Btheta_2\|\leq\varpi/(p_t\sigma_e^2\bar f)$ and thus $\|\Psi\left(\Bx_0;\Btheta_1,\Bmeta^{\star}(\Bx_0)\right)-\Psi\left(\Bx_0;\Btheta_2,\Bmeta^{\star}(\Bx_0)\right)\|\leq\varpi$. Then the bracketing entropy $\log N_{[]}\left(\varpi,\Psi,L_2 \right) $ is bounded by $O\left(\varpi^{-1} \right) $. Similar to Lemma 9 in \cite{athey2019generalized}, we have $\left\| \delta\left((\Btheta^{\star}(\Bx_0),\Bmeta^{\star}(\Bx_0)),(\widehat{\Btheta}(\Bx_0),\Bmeta^{\star}(\Bx_0))\right) \right\|=O_p\left((s/n)^{\frac{2}{3}}\right)$.

For the next four terms, we have $\left\|\Psi(\Bx_0;\widehat{\Btheta}(\Bx_0),\Bmeta^{\star}(\Bx_0)) \right\|=O(\frac{s}{n})$ by Assumption~\ref{A3.7}. According to Proposition~\ref{thm:nuisance_error} and Theorem~\ref{thm_conv}, $\left\|\Psi_0(\Bx_0;\Btheta^{\star}(\Bx_0),\Bmeta^{\star}(\Bx_0)) \right\|=O_p\left(s^{-\frac{1}{2\omega p_x}}+\frac{s\log(p_t+p_w)}{n}\right)$. Proposition~\ref{thm:shrinkage} implies that the second to the last term is $O_p(s^{-\frac{1}{2\omega p_x}})$. The last term is of order $O\left(\left\|\Bmeta^{\star}(\Bx_0)-\widetilde{\Bmeta}(\Bx_0)\right\|^2\right)$ by the orthogonality. Since $s=O(n^b)$ with $b\in(1-\frac{1}{1+\omega p_x},1)$, it follows that $s^{-\frac{1}{2\omega p_x}}=o\left(\left(\frac{s}{n}\right)^{\frac{1}{2}}\right)$ and thus this term can be ignored. Therefore the conclusion in Theorem 3 holds.
\end{proof}

\bibliographystyle{elsarticle-harv}
\bibliography{ref}
\end{document}
